# Supplementary material for: Estimating Functionals of the Joint Distribution of Potential Outcomes with Optimal Transport
Source: arXiv:2311.09435 source file (2023-11-15)
Supplement: Supplementary file 1 [file OTJointPO_appendix_inference_AvoidBootstrap.tex]

\newpage
\section*{Avoiding the bootstrap}

UNFINISHED; CUT?

Although simple, the bootstrap can become time consuming when the sample size is large. The reason is solving linear programming problems for each bootstrap iteration. This section describes a consistent alternative that avoids computing these problems for each bootstrap iteration, and should work when treatment is exogenous.

The idea is to immitage the proof of \ref{Theorem: inference, bootstrap, Fang and Santos alternative works}, but to replace the more complex $\widehat{OT}_{c,x}'(H_{1,x}, H_{0,x})$ with the simpler $\widehat{OT}_{c, (\hat{P}_{1 \mid x}, \hat{P}_{0 \mid x})}'(H_{1,x}, H_{0,x})$. 
\begin{enumerate}
	\singlespacing
	\item Solve the numerical programming problem, obtaining solutions $(\hat{\varphi}_{c_L ,x}, \hat{\psi}_{c_L,x}) \in \mathcal{F}_c \times \mathcal{F}_c^c$ and $(\hat{\varphi}_{c_H ,x}, \hat{\psi}_{c_H,x}) \in \mathcal{F}_c \times \mathcal{F}_c^c$ for each $x \in \mathcal{X}$
	\begin{itemize}
		\item To enforce the solutions are in $\mathcal{F}_c \times \mathcal{F}_c^c$, with exogenous treatment we can just take $c$-transforms of the solutions.
		\item To ensure the solution is unique, set $\sup_y \psi_{c,x}(y) = 0$ for each $(c,x)$. This is easily enforced by simply adding a constant to $\hat{\psi}_{c,x}$ before taking $c$-transforms.
	\end{itemize}
	
	\item Define $\widehat{OT}_{c, (\hat{P}_{1 \mid x}, \hat{P}_{0 \mid x})} : \mathcal{C}(\mathcal{F}_c \times L_{2,P}) \times \mathcal{C}(\mathcal{F}_c^c \times L_{2,P})$ with
	\begin{align*}
		\widehat{OT}_{c, (\hat{P}_{1 \mid x}, \hat{P}_{0 \mid x})}'(H_{1,x}, H_{0,x}) = H_{1,x}(\hat{\varphi}_{c ,x}) + H_{0,x}(\hat{\psi}_{c,x})
	\end{align*}
	and $\widehat{T}_{2,T_1(P)}(\cdot)$ largely the same as in section \ref{Section: estimators, subsection inference, subsubsection consistent alternative}:
	\begin{align*}
		&\widehat{T}_{2,T_1(P)}'\left(\{H_{1,x}, H_{0,x}, h_{\eta_1, x}, h_{\eta_0, x}, h_{s, x}\}_{x \in \mathcal{X}}\right) \\
		&\hspace{1 cm} = \left(\left\{\widehat{OT}_{c_L, (\hat{P}_{1 \mid x}, \hat{P}_{0 \mid x})}'(H_{1,x}, H_{0,x}), -\widehat{OT}_{c_H, (\hat{P}_{1 \mid x}, \hat{P}_{0 \mid x})}'(H_{1,x}, H_{0,x}), h_{\eta_1, x}, h_{\eta_0, x}, h_{s, x}\right\}_{x \in \mathcal{X}}\right)
	\end{align*}
	\item Estimate the asymptotic distribution with the conditional law of 
	\begin{equation*}
		\hat{D}_4 \hat{D}_3 \widehat{T}_{2, T_1(P)}'\left(\sqrt{n}(T_1(\mathbb{P}_n^*) - T_1(\mathbb{P}_n))\right)
	\end{equation*}
	with $T_1$, $\hat{D}_4$, and $\hat{D}_3$ exactly as defined in section \ref{Section: estimators, subsection inference, subsubsection consistent alternative}. 
\end{enumerate}

Notice that 
\begin{align*}
	&\sqrt{n}(T_1(\mathbb{P}_n^*) - T_1(\mathbb{P}_n)) \\
	&\hspace{1 cm} = \sqrt{n}\left\{\hat{P}_{1 \mid x}^* - \hat{P}_{1 \mid x}, \hat{P}_{0 \mid x}^* - \hat{P}_{0 \mid x}, \hat{\eta}_{1, x}^* - \hat{\eta}_{1, x}, \hat{\eta}_{0, x}^* - \hat{\eta}_{0,x}, \hat{s}_x^* - \hat{s}_x\right\}_{x \in \mathcal{X}}
\end{align*}

The major computational savings here is that for each bootstrap iteration, we simply need to compute (being loose with notation here):
\begin{align*}
	&\widehat{OT}_{c_L, (\hat{P}_{1 \mid x}, \hat{P}_{0 \mid x})}'(\sqrt{n}(\hat{P}_{1 \mid x}^* - \hat{P}_{1 \mid x}), \sqrt{n}(\hat{P}_{0 \mid x}^* - \hat{P}_{0 \mid x})) \\
	&\hspace{1 cm} = \sqrt{n}(\hat{P}_{1 \mid x}^*(\hat{\varphi}_{c_L,x}) + \hat{P}_{0 \mid x}^*(\hat{\psi}_{c_L,x}) - \hat{P}_{1 \mid x}(\hat{\varphi}_{c_L,x}) - \hat{P}_{0 \mid x}(\hat{\psi}_{c_L,x})) \\
	&\hspace{1 cm} = \sqrt{n}(\widehat{OT}_{c_L, (\hat{P}_{1 \mid x}, \hat{P}_{0 \mid x})}'(\hat{P}_{1\mid x}^*, \hat{P}_{0 \mid x}^*) - \widehat{OT}_{c_L, (\hat{P}_{1 \mid x}, \hat{P}_{0 \mid x})}'(\hat{P}_{1\mid x}, \hat{P}_{0 \mid x}))
\end{align*}
and similar for $c_H$, for each $x \in \mathcal{X}$. This is instead of solve another set of linear programming problems.

To simplify the coding, note that 
\begin{align*}
	&\hat{D}_4 \hat{D}_3 \widehat{T}_{2, T_1(P)}'\left(\sqrt{n}(T_1(\mathbb{P}_n^*) - T_1(\mathbb{P}_n))\right) \\
	&\hspace{1 cm} = 
\end{align*}

To argue this works,	
\begin{enumerate}
	\item The same argument as the proof of theorem \ref{Theorem: inference, bootstrap, Fang and Santos alternative works} will work, once we show that for each fixed $(H_{1,x}, H_{0,x}) \in  \mathcal{C}(\mathcal{F}_c \times L_{2,P}) \times \mathcal{C}(\mathcal{F}_c^c \times L_{2,P})$,
	\begin{equation*}
		\widehat{OT}_{c,(\hat{P}_{1 \mid x}, \hat{P}_{0 \mid x})}'(H_{1,x}, H_{0,x}) \overset{p}{\rightarrow} OT_{c(P_{1\mid x}, P_{0\mid x})}'(H_{1,x}, H_{0,x})
	\end{equation*}
	
	\item Apply \cite{van2000asymptotic} theorem 5.7 to find that $(\hat{\varphi}_{c,x}, \hat{\psi}_{c,x}) \overset{p}{\rightarrow} (\varphi_{c,x}, \psi_{c,x})$ in $L_{2,P} \times L_{2,P}$. 
	\begin{itemize}
		\item Use compactness to obtain well-separated
	\end{itemize}
	
	\item Then use continuity: $(H_{1,x}, H_{0,x})$ is continuous in $L_{2,P} \times L_{2,P}$, so 
	\begin{align*}
		&\widehat{OT}_{c,(\hat{P}_{1 \mid x}, \hat{P}_{0 \mid x})}'(H_{1,x}, H_{0,x}) \\
		&\hspace{1 cm} = H_{1,x}(\hat{\varphi}_{c ,x}) + H_{0,x}(\hat{\psi}_{c,x}) \overset{p}{\rightarrow} H_{1,x}(\varphi_{c ,x}) + H_{0,x}(\psi_{c,x}) \\
		&\hspace{1 cm} = OT_{c(P_{1\mid x}, P_{0\mid x})}'(H_{1,x}, H_{0,x})
	\end{align*}
\end{enumerate}

We'll test this on the following parameter from example \ref{Example: equitable policies}:
\begin{align*}
	\gamma &= g(\theta, \eta) = g(\theta, \eta_1, \eta_0) \\
	&= \frac{\text{Cov}(Y_1 - Y_0, Y_0)}{\text{Var}(Y0)} \\
	&= \frac{E_{P_{1,0}}[(Y_1 - Y_0) Y_0] - (E_{P_1}[Y_1] - E_{P_0}[Y_0])E_{P_0}[Y_0]}{E_{P_0}[Y_0^2] - (E_{P_0}[Y_0])^2}
\end{align*}
Here the functions are
\begin{align*}
	\eta_1(Y_1) &= Y_1 \\
	\eta_0(Y_0) &= (Y_0, Y_0^2) \\
	g(t,e_1,e_0) &= \frac{t - (e_1 - e_0^{(1)})e_0^{(1)}}{e_0^{(2)} - (e_0^{(1)})^2}
\end{align*}
and since $g^L(t_1, t_0, e_1, e_0) = \inf_{t \in [t_1, t_0]} g(t, e_1, e_0) = g(t_L, e_1, e_0)$, we have
\begin{align*}
	\nabla g^L(t_1, t_0, e_1, e_0) &= \begin{pmatrix}
		g_t (t_L, e_1,e_0) & 0 & g_{e_1} (t_L, e_1,e_0) & g_{e_0} (t_L, e_1,e_0)
	\end{pmatrix} 
\end{align*}
where
\begin{align*}
	g_t(t_L, e_1, e_0) &= \frac{1}{e_0^{(2)} - (e_0^{(1)})^2} \\
	g_{e_1}(t_L, e_1, e_0) &= \frac{-e_0^{(1)}}{e_0^{(2)} - (e_0^{(1)})^2} \\
	g_{e_0}(t_L, e_1, e_0) &= 
	\begin{pmatrix}
		\frac{2e_0^{(1)}(t_L + e_0^{(2)}) - e_1((e_0^{(1)})^2 + e_0^{(2)})}{(e_0^{(2)} - (e_0^{(1)})^2)^2} & 
		\frac{e_0^{(1)}(e_1 - e_0^{(1)}) - t_L}{(e_0^{(2)} - (e_0^{(1)})^2)^2}
	\end{pmatrix}	
\end{align*}

\newpage
