# Supplementary material for: Estimating Functionals of the Joint Distribution of Potential Outcomes with Optimal Transport
Source: arXiv:2311.09435 source file (2023-11-15)
Supplement: Supplementary file 2 [file OTJointPO_appendix_instruments_messy.tex]

\section{Instruments (MESSY)}
\label{Appendix: Instruments (Messy)}
\begin{singlespace}
	\begin{mdframed}
		This section contains sketches investigating how instruments could be incorporated, using essentially the LATE framework.
		
		This space contains sketches to figure out whether it works, and the best way to incorporate them into the framework.
	\end{mdframed}
	
	Suppose the econometrician observes an i.i.d. sample $\{Y_i, D_i, Z_i, X_i\}_{i=1}^n$ with 
	\begin{align}
		&Y \in \mathbb{R}, &&D \in \{0,1\}, &&Z \in \{0,1\}, &&X_i \in \mathcal{X} = \{x_1, \ldots, x_M\} \label{Display: LATE IV setup}
	\end{align}
	where $Y$ is an outcome of interest, $D$ indicates treatment status, and $Z$ is a binary instrument assumed to affect treatment status. Assume the LATE framework: $D$ is related to potential treatment statuses $D_1, D_0 \in \{0,1\}$ and $Y$ to potential outcomes $Y_1, Y_0 \in \mathbb{R}$ by
	\begin{align}
		&D = ZD_1 + (1-Z) D_0, &&Y = D Y_1 + (1-D) Y_0 \label{Display: LATE IV observed and potential treatment statuses and outcomes}
	\end{align}
	Furthermore, assume that conditional on covariates the instrument is independent of potential outcomes and treatment statuses:
	\begin{equation}
		(Y_1, Y_0, D_1, D_0) \perp Z \mid X \label{Display: LATE IV instrument exogeneity}
	\end{equation}
	Notice this is implied by the stronger $(Y_1, Y_0, D_1, D_0, X) \perp Z$.\footnote{
		Sketch: For any $z \in \{0,1\}$ and any set $A \in \mathbb{R} \times \mathbb{R} \times \{0,1\} \times \{0,1\}$,
		\begin{align*}
			P(Z = z, (Y_1, Y_0, D_1, D_0) \in A \mid X = x) &= P(Z = z \mid (Y_1, Y_0, D_1, D_0) \in A, X = x)P((Y_1, Y_0, D_1, D_0) \in A \mid X = x) \\
			&= P(Z = z \mid X = x)P((Y_1, Y_0, D_1, D_0) \in A \mid X = x) \\
		\end{align*}
	}
	Finally, assume \textit{monotonicity}:
	\begin{equation}
		D_1 \geq D_0 \text{ almost surely } \label{Display: LATE IV monotonicity}
	\end{equation}
	The direction of monotonicity is without loss of generality.\footnote{If $D_0 \geq D_1$ almost surely, simply define $\tilde{Z} = 1- Z$ and note that $D_{\tilde{z} = 1} \geq D_{\tilde{z} = 0}$.} 
	
	Finally, assume $P(D = d, Z = z, X = x) > 0$ for all $(d,z,x)$, and that the instrument has a positive probability of changing the treatment status: $P(D_1 \neq D_0) > 0$.
	
	\subsection{Identification}
	
	\subsubsection{Without covariates}

	Suppose there are no covariates; the sample is $\{Y_i, D_i, Z_i\}_{i=1}^n$, and identifies 4 conditional distributions and 4 probabilities: for all $(d,z)$,
	\begin{align*}
		&Y \mid D = d, Z = z &&p_{dz} = P(D = d, Z = z)
	\end{align*}
	
	The primitives are $(Y_1, Y_0, D_1, D_0, Z)$. The following is identified:
	\begin{align*}
		&\text{Conditional distributions}
		\begin{cases}
			Y_d \mid D_1 = 1, D_0 = 1, Z = z\\
			Y_d \mid D_1 = 1, D_0 = 0, Z = z \\
			Y_d \mid D_1 = 0, D_0 = 0, Z = z
		\end{cases},
		&&\text{Probabilities}
		\begin{cases}
			P(D_1 = 1, D_0 = 1, Z = z) \\
			P(D_1 = 1, D_0 = 0, Z = z) \\
			P(D_1 = 0, D_0 = 0, Z = z)
		\end{cases}
	\end{align*}
	
	THERE'S A MISTAKE HERE; THERE'S NO WAY THE DISTRIBUTION OF $Y_0$ CONDITIONAL ON BEING AN ALWAYS-TAKER IS IDENTIFIED.
	
	Since the monotonicity assumption implies $P(D_1 = 0, D_1 = 1, Z = z) = 0$, there is no meaningful distribution of $Y_d \mid D_1 = 0, D_1 = 1, Z = z$. 
	\begin{enumerate}
		\item The distribution of $(D_1, D_0, Z)$ is identified.
		
		Monotonicity (assumption \eqref{Display: LATE IV monotonicity}) implies the random variable $\mathbbm{1}\{D_1 = 0, D_ 0 = 1\}$ equals zero. This implies
		\begin{align*}
			\mathbbm{1}\{D_1 = 1\} = \mathbbm{1}\{D_1 = 1, D_0 = 1\} + \mathbbm{1}\{D_1 = 1, D_0 = 0\} \\
			\mathbbm{1}\{D_1 = 0\} = \cancel{\mathbbm{1}\{D_1 = 0, D_0 = 1\}} + \mathbbm{1}\{D_1 = 0, D_0 = 0\} \\
			\mathbbm{1}\{D_0 = 1\} = \mathbbm{1}\{D_1 = 1, D_0 = 1\} + \cancel{\mathbbm{1}\{D_1 = 0, D_1 = 1\}} \\
			\mathbbm{1}\{D_0 = 0\} = \mathbbm{1}\{D_1 = 1, D_0 = 0\} + \mathbbm{1}\{D_1 = 0, D_0 = 0\} \\
		\end{align*}
		where cancelled terms are (almost surely) equal to zero. Taking expectations and using assumption \eqref{Display: LATE IV instrument exogeneity} we obtain
		\begin{align*}
			P(D = 1 \mid Z = 1) &= P(D_1 = 1) = P(D_1 = 1, D_0 = 1) + P(D_1 = 1, D_0 = 0) \\
			P(D = 0 \mid Z = 1) &= P(D_1 = 0) = P(D_1 = 0, D_0 = 0) \\
			P(D = 1 \mid Z = 0) &= P(D_0 = 1) = P(D_1 = 1, D_0 = 1) \\
			P(D = 0 \mid Z = 0) &= P(D_0 = 0) = P(D_1 = 1, D_0 = 0) + P(D_1 = 0, D_0 = 0)
		\end{align*}
		Finally, use these to see that 
		\begin{align}
			P(D_1 = 1, D_0 = 0) &= P(D = 1 \mid Z = 1) - P(D = 1 \mid Z = 0) \label{Display: LATE IV, compliers D=1} \\
			&= P(D = 0 \mid Z = 0) - P(D = 0 \mid Z = 1) \label{Display: LATE IV, compliers D=0} \\
			&= 1 - P(D = 0 \mid Z = 1) - P(D = 1 \mid Z = 0) \label{Display: LATE IV, compliers through complement}
		\end{align}
		since $P(D_1 = 0, D_1 = 0) = 0$ by assumption, the distribution of $(D_1, D_0)$ is identified. Since $Z$ is independent of $(D_1, D_0)$ and $P(Z = z)$ is identified, the distribution of $(D_1, D_0, Z)$ is identified.\footnote{		
			Aside: these are equivalent:
			\begin{align*}
				P(D = 0 \mid Z = 0) - P(D = 0 \mid Z = 1) &= E[(1-D) \mid Z = 0] - E[(1-D) \mid Z = 1] \\
				&= 1 - P(D = 1 \mid Z = 0) - 1 + P(D = 1 \mid Z = 1) \\
				&= P(D = 1 \mid Z = 1) - P(D = 1 \mid Z = 0)
			\end{align*}
			and furthermore,
			\begin{align*}
				&1 - P(D = 0 \mid Z = 1) - P(D = 1 \mid Z = 0) \\
				&\hspace{1 cm} = \frac{1}{2}\left[P(D = 1 \mid Z = 1) + P(D = 0 \mid Z = 1) + P(D = 1 \mid Z = 0) + P(D = 0 \mid Z = 0) \right] \\
				&\hspace{2 cm} - P(D = 0 \mid Z = 1) - P(D = 1 \mid Z = 0) \\
				&\hspace{1 cm} = \frac{1}{2}\left[P(D = 1 \mid Z = 1) - P(D = 1 \mid Z = 0) + P(D = 0 \mid Z = 0) - P(D = 1 \mid Z = 0)\right]
			\end{align*}
		}
		
		\item The distribution of $(Y_d, D_z, Z)$ is identified. 
		
		Assumption \eqref{Display: LATE IV instrument exogeneity} simplifies to $(Y_1, Y_0, D_1, D_0) \perp Z$, and along with \eqref{Display: LATE IV observed and potential treatment statuses and outcomes} implies that
		\begin{align*}
			&Y \mid D = d, Z = z &&\text{ has the same distribution as } &&Y_d \mid D_z = d
		\end{align*}
		and, since $P(Y_d \in A \mid D_z = d, Z = z') = P(Y_d \in A \mid D_z = d)$, we have also have 
		\begin{equation*}
			P(Y_d \in A \mid D_z = d, Z = z') = P(Y_d \in A \mid D_z = d, Z = z) = P(Y \in A \mid D = d, Z = z)
		\end{equation*}
		This implies the whole distribution of $(Y_d, D_z, Z)$ is identified:
		\begin{align*}
			P(Y_d \in A, D_z = d, Z = z') &= P(Y_d \in A \mid D_z = d, Z = z') P(D_z = d \mid Z = z')P(Z = z') \\
			&= P(Y_d \in A \mid D_z = d, Z = z) P(D_z = d \mid Z = z)P(Z = z') \\
			&= P(Y \in A \mid D = d, Z = z) P(D = d \mid Z = z) P(Z = z')
		\end{align*}
		Notice that monotonicity implies 
		\begin{align*}
			&Y_d \mid D_1 = 0, Z = z &&\text{ has the same distribution as } &&Y_d \mid D_1 = 0, D_0 = 0, Z = z \\
			&Y_d \mid D_0 = 1, Z = z &&\text{ has the same distribution as } &&Y_d \mid D_1 = 1, D_0 = 1, Z = z
		\end{align*}
		
		\item The distribution of $Y_d \mid D_1 = 1, D_0 = 0, Z = z$, sometimes denoted $Y_d \mid D_1 > D_0, Z = z$, is identified.
		
		Notice that monotonicity implies
		\begin{align*}
			\mathbbm{1}\{D_1 = 1\} - \mathbbm{1}\{D_0 = 1\} &= \underbrace{\mathbbm{1}\{D_1 = 1, D_0 = 0\} + \mathbbm{1}\{D_1 = 1, D_0 = 1\}}_{=\mathbbm{1}\{D_1 = 1\}} \\
			&\hspace{1 cm} - \underbrace{\left(\mathbbm{1}\{D_1 = 1, D_0 = 1\} + \cancel{\mathbbm{1}\{D_1 = 0, D_0 = 1\}}\right)}_{=\mathbbm{1}\{D_0 = 1\}} \\
			&= \mathbbm{1}\{D_1 = 1, D_0 = 0\} = \mathbbm{1}\{D_1 > D_0\}
		\end{align*}
		and similarly,
		\begin{align*}
			\mathbbm{1}\{D_0 = 0\} - \mathbbm{1}\{D_1 = 0\} &= \underbrace{\left(\mathbbm{1}\{D_1 = 1, D_0 = 0\} + \mathbbm{1}\{D_1 = 0, D_0 = 0\}\right)}_{= \mathbbm{1}\{D_0 = 0\}} \\
			&\hspace{1 cm} -  \underbrace{\mathbbm{1}\{D_1 = 0, D_0 = 0\} + \cancel{\mathbbm{1}\{D_1 = 0, D_0 = 1\}}}_{=\mathbbm{1}\{D_1 = 0\}} \\
			&= \mathbbm{1}\{D_1 = 1, D_0 = 0\} = \mathbbm{1}\{D_1 > D_0\}
		\end{align*}
		We could proceed considering the probability $Y_d \in A$, but eventually we'll want to evaluate expectations. So instead consider an arbitrary function $f$, and note that
		\begin{align*}
			&E[f(Y)D \mid Z = 1] - E[f(Y) D \mid Z = 0] \\
			&\hspace{1 cm} = E[f(D_1 Y_1 + (1-D_1)Y_0)D_1] - E[f(D_0 Y_1 + (1-D_0)Y_0) D_0] \\
			&\hspace{1 cm} = E[f(Y_1) \mathbbm{1}\{D_1 = 1\}] - E[f(Y_1) \mathbbm{1}\{D_0 = 1\}] \\
			&\hspace{1 cm} = E[f(Y_1) (\mathbbm{1}\{D_1 = 1\} - \mathbbm{1}\{D_0 = 1\})] \\
			&\hspace{1 cm} = E[f(Y_1) \mathbbm{1}\{D_1 > D_0\}] \\
			&\hspace{1 cm} = E[f(Y_1) \mid D_1 > D_0] P(D_1 > D_0) 
		\end{align*}
		Similarly,
		\begin{align*}
			E[f(Y)(1-D) \mid Z = 0] - E[f(Y) (1-D) \mid Z = 1] &= E[f(Y_0)(1-D_0)] - E[f(Y_0)(1-D_1)] \\
			&= E[f(Y_0) \mathbbm{1}\{D_0 = 0\}] - E[f(Y_0) \mathbbm{1}\{D_1 = 0\}] \\
			&= E[f(Y_0)(\mathbbm{1}\{D_0 = 0\} - \mathbbm{1}\{D_1 = 0\})] \\
			&= E[f(Y_0) \mid D_1 > D_0]P(D_1 > D_0)
		\end{align*}
		since $P(D_1 > D_0) = P(D_1 = 1, D_0 = 0)$ is identified (see \eqref{Display: LATE IV, compliers D=1} and \eqref{Display: LATE IV, compliers D=0} above), we can compute 
		\begin{align*}
			E[f(Y_1) \mid D_1 > D_0] &= \frac{E[f(Y)D \mid Z = 1] - E[f(Y) D \mid Z = 0]}{P(D = 1 \mid Z = 1) - P(D = 1 \mid Z = 0)}, \\
			& \\
			E[f(Y_0) \mid D_1 > D_0] &= \frac{E[f(Y)(1-D) \mid Z = 0] - E[f(Y) (1-D) \mid Z = 1]}{P(D = 0 \mid Z = 0) - P(D = 0 \mid Z = 1)} 
		\end{align*}
		
		This shows the distribution of $Y_d \mid D_1 = 1, D_0 = 0$ is identified. Since assumption \eqref{Display: LATE IV instrument exogeneity} implies $(Y_1, Y_0, D_1, D_0) \perp Z$, the distribution of $Y_d \mid D_1 = 1, D_0 = 0, Z = z$ is identified as well.
	\end{enumerate}

	The model is (quite) overidentified. As discussed in \cite{kitagawa2015test}, the identification of $Y_d \mid D_1 = 1, D_0 = 0$ implies that for any set $B$,
	\begin{align*}
		P(Y \in B, D = 1 \mid Z = 1) \geq P(Y \in B, D = 1 \mid Z = 0) \\
		P(Y \in B, D = 0 \mid Z = 0) \geq P(Y \in B, D = 0 \mid Z = 1)
	\end{align*}
	
	The important question for our purposes: supposing the identified information doesn't already contradict the model (i.e., the inequalities above hold for all $B$),
	\begin{center}
		\textbf{Can $(Y_1, Y_0) \mid D_1 = 1, D_0 = 0$ take any copula?}
	\end{center}
	In other words, given a distribution $P_{Y,D,Z}$ of $(Y, D, Z)$ that doesn't contradict the model and an arbitrary coupling of $Y_1 \mid D_1 = 1, D_0 = 0$ and $Y_0 \mid D_1 = 1, D_0 = 0$, is there a distribution of the primitives with that coupling that doesn't contradict the model?
	
	I think so. Just as in the proof of lemma \ref{Lemma: identification, function of moments}, for any set $A$ 
	\begin{align*}
		&P((Y_1, Y_0) \in A, D_1 = d_1, D_0 = d_0, Z = z) \\
		&\hspace{1 cm} = P((Y_1, Y_0) \in A \mid D_1 = d_1, D_0 = d_0, Z = z)P(D_1 = d_1, D_0 = d_0)P(Z = z)
	\end{align*}
	supposing that $d_1 = 1$ and $d_0 = 0$, and the model is not already rejected by the distribution of $(Y, D, Z)$, I don't see how any copula could get us into trouble. It would have the right marginals, and thus ``match'' the identified information - which is already assumed to not contradict the model.

	\subsubsection{With covariates}
	
	Do any of the arguments above break with covariates? I don't think so.
	
	The primitives of the model are $(Y_1, Y_0, D_1, D_0, Z, X)$. The i.i.d. sample identifies the distribution of $(Y, D, Z, X)$, which can be broken into the $4M$ probabilities $p_{dxz} = P(D = d, X = x, Z = z)$. For each probability that is positive, we have a corresponding conditional distribution:
	\begin{align*}
		Y \mid D = d, X = x, Z = z
	\end{align*}
	
	We'll need to strengthen assumption \ref{Assumption: setting} \ref{Assumption: setting, common support} to 
	\begin{equation*}
		P(D = 1, Z = 1, X = x) > 0 \text{ and } P(D = 0, Z = 0, X = x) > 0 \text{ for all } x \in \mathcal{X}
	\end{equation*}
	But it is fine if $P(D = 0, Z = 1, X = x) = 0$ or $P(D = 1, Z = 0, X = x) = 0$; the former simply implies there are no never-takers and the latter that there are no always-takers. 
	
	Note that $D_1 \geq D_0$ almost surely and $P(X = x) > 0$ implies that $\mathbbm{1}\{D_1 = 0, D_0 = 1, X = x\}$ equals zero (almost surely). Otherwise, we'd have the contradiction
	\begin{align*}
		P(D_1 < D_0) = \sum_x P(D_1 < D_0 \mid X = x)P(X = x) > 0
	\end{align*}
	This implies
	\begin{align*}
		\mathbbm{1}\{D_1 = 1, X = x\} &= \mathbbm{1}\{D_1 = 1, D_0 = 1, X = x\} + \mathbbm{1}\{D_1 = 1, D_0 = 0, X = x\} \\
		\mathbbm{1}\{D_1 = 0, X = x\} &= \cancel{\mathbbm{1}\{D_1 = 0, D_0 = 1, X = x\}} + \mathbbm{1}\{D_1 = 0, D_0 = 0, X = x\} \\
		\mathbbm{1}\{D_0 = 1, X = x\} &= \mathbbm{1}\{D_1 = 1, D_0 = 1, X = x\} + \cancel{\mathbbm{1}\{D_1 = 0, D_0 = 1, X = x\}} \\
		\mathbbm{1}\{D_0 = 0, X = x\} &= \mathbbm{1}\{D_1 = 1, D_0 = 0, X = x\} + \mathbbm{1}\{D_1 = 0, D_0 = 0, X = x\}
	\end{align*}
	Taking expectations and dividing by $P(X = x)$ gives
	\begin{align*}
		P(D_1 = 1 \mid X = x) &= P(D_1 = 1, D_0 = 1 \mid X = x) + P(D_1 = 1, D_0 = 0 \mid X = x) \\
		P(D_1 = 0 \mid X = x) &= P(D_1 = 0, D_0 = 0 \mid X = x) \\
		P(D_0 = 1 \mid X = x) &= P(D_1 = 1, D_0 = 1 \mid X = x) \\
		P(D_0 = 0 \mid X = x) &= P(D_1 = 1, D_0 = 0 \mid X = x) + P(D_1 = 0, D_0 = 0 \mid X = x)
	\end{align*}
	Finally, note that 
	\begin{align*}
		P(D = 1 \mid Z = 1, X = x) &= P(D_1 = 1 \mid X = x) \\
		P(D = 0 \mid Z = 1, X = x) &= P(D_1 = 0 \mid X = x) \\
		P(D = 1 \mid Z = 0, X = x) &= P(D_0 = 1 \mid X = x) \\
		P(D = 0 \mid Z = 0, X = x) &= P(D_0 = 0 \mid X = x) 
	\end{align*}
	and thus the share of compliers conditional on $X = x$ can be computed with (any) of the three (equivalent) formulas:
	\begin{align*}
		P(D_1 > D_0 \mid X = x) &= P(D_1 = 1, D_0 = 0 \mid X = x) \\
		&= P(D = 1 \mid Z = 1, X = x) - P(D = 1 \mid Z = 0, X = x) \\
		&= P(D = 0 \mid Z = 0, X = x) - P(D = 0 \mid Z = 1, X = x) \\
		&= 1 - P(D = 0 \mid Z = 1, X = x) - P(D = 1 \mid Z = 0, X = x)
	\end{align*}
	
	Finally, note that 
	\begin{align*}
		&\mathbbm{1}\{D_1 = 1, X = x\} - \mathbbm{1}\{D_0 = 1, X = x\} = \mathbbm{1}\{D_1 = 1, D_0 = 0, X = x\} \\
		&\hspace{1 cm} = \mathbbm{1}\{D_1 > D_0\}\mathbbm{1}\{X = x\} 
	\end{align*}
	Implying that 
	\begin{align*}
		&E[f(Y)D \mid Z = 1, X = x] - E[f(Y)D \mid Z = 0, X = x] \\
		&\hspace{1 cm} = E[f(D_1Y_1 + (1-D_1)Y_0)D_1 \mid Z = 1, X = x] - E[f(D_0 Y_1 + (1-D_0)Y_0)D_0 \mid Z = 0, X = x] \\
		&\hspace{1 cm} = E[f(Y_1)D_1 \mid X = x] - E[f(Y_1)D_0 \mid X = x] \\
		&\hspace{1 cm} = E[f(Y_1)(\mathbbm{1}\{D_1 = 1\} - \mathbbm{1}\{D_0 = 1\}) \mid X = x] \\
		&\hspace{1 cm} = E[f(Y_1) \mathbbm{1}\{D_1 > D_0\} \mid X = x] \\
		&\hspace{1 cm} = E[f(Y_1) \mid D_1 > D_0, X = x] P(D_1 > D_0 \mid X = x)
	\end{align*}
	
	In other words, the same tricks used above work to show
	\begin{align*}
		&E[f(Y)D \mid Z= 1, X = x] - E[f(Y)D \mid Z = 0, X = x] \\
		&\hspace{2 cm} = E[f(Y_1) \mid D_1 > D_0, X = x]P(D_1 > D_0 \mid X = x) \\
		&E[f(Y)(1-D) \mid Z= 1, X = x] - E[f(Y)(1-D) \mid Z = 0, X = x] \\
		&\hspace{2 cm} = E[f(Y_0) \mid D_1 > D_0, X = x]P(D_1 > D_0 \mid X = x) 
	\end{align*}
	Which implies the conditional distributions of $Y_d$ conditional on being a complier are given by
	\begin{align*}
		E[f(Y_1) \mid D_1 > D_0, X = x] &= \frac{E[f(Y)D \mid Z = 1, X = x] - E[f(Y) D \mid Z = 0, X = x]}{P(D = 1 \mid Z = 1, X = x) - P(D = 1 \mid Z = 0, X = x)}, \\
		& \\
		E[f(Y_0) \mid D_1 > D_0, X = x] &= \frac{E[f(Y)(1-D) \mid Z = 0, X = x] - E[f(Y) (1-D) \mid Z = 1, X = x]}{P(D = 0 \mid Z = 0, X = x) - P(D = 0 \mid Z = 1, X = x)} 
	\end{align*}

	\newpage
	
	\subsection{Estimation}
	
	The idea is to use sample analogues to these expressions:
	\begin{align*}
		E[f(Y_1) \mid D_1 > D_0, X = x] &= \frac{E[f(Y)D \mid Z = 1, X = x] - E[f(Y) D \mid Z = 0, X = x]}{P(D = 1 \mid Z = 1, X = x) - P(D = 1 \mid Z = 0, X = x)}, \\
		& \\
		E[f(Y_0) \mid D_1 > D_0, X = x] &= \frac{E[f(Y)(1-D) \mid Z = 0, X = x] - E[f(Y) (1-D) \mid Z = 1, X = x]}{P(D = 0 \mid Z = 0, X = x) - P(D = 0 \mid Z = 1, X = x)} 
	\end{align*}
	Begin by noticing that we can start with the same large Donsker set, now multiplied by additional (but a finite number of) indicators. So it remains Donsker (see lemma \ref{Lemma: weak convergence, large Donsker set is Donsker} section \ref{Appendix: weak convergence}).

	\subsection{Planning: rewrite using dominated distributions (24 August 2023)}
	
	We can rewrite the main results to working with a dominating distribution. This will make it easier to show the limiting distribution of the ``first step'' (constructing conditional distributions) is supported in the set of functions that are continuous with respect to this dominating $L_2$ semimetric.
	
	\begin{mdframed}
		Here's the actual steps we'll take, which are sketched below:
		\begin{enumerate}
			\item Section \ref{Section: identification} may change significantly to accomodate the LATE IV framework, but a lot will probably stay.
			\begin{itemize}
				\item With exogenous treatment we get unconditional parameters. These are easier to understand, motivate, and the identification is easier to see - so the example should stay as it is, with exogenous treatment.
				\item With LATE IV, we get parameters conditional on being a complier. We should cite \cite{imbens1994late}, and note that these are especially of interest if the policy decision to be made is to assign everyone the instrument; i.e. set $Z = 1$. The subpopulation swayed by the instrument is exactly the distribution we're studying. 
				\item The parameter assumptions can stay as they are; once we've defined $P_{1 \mid x}$ and $P_{0 \mid x}$, much of the analysis remains the same. 
			\end{itemize}
			
			\item Section \ref{Section: duality and differentiability} (duality and differentiability) should be essentially emptied out. There isn't much there, and it'll change.
			\begin{itemize}
				\item The $L_2$ semimetrics in section \ref{Section: duality and differentiability} will no longer be relevant; cut them and replace them with $L_{2,P}$. Note the ambiguity in $P$: when treatment is exogenous, $(Y,D, X) \sim P$ and in the LATE IV framework, $(Y, D, Z, X) \sim P$. 
			\end{itemize}
			
			\item Rewrite appendix \ref{Appendix: properties of optimal transport}:
			\begin{enumerate}
				\item Start with subsection \ref{Appendix: properties of optimal transport, subsection differentiability}: cut discussion of the tangent set, and rewrite lemmas \ref{Lemma: Hadamard differentiability, optimal transport} and \ref{Lemma: Hadamard differentiability, optimal transport, particular cases}.
				\item In subsection \ref{Appendix: properties of optimal transport, subsection differentiability, subsubsection full differentiability}, introduce a new concept: the subset of $\ell^\infty(\mathcal{F})$ that is linear and evaluates constant functions to zero. Currently, the notation is $\ell_{Lin, zero}^\infty(\mathcal{F})$. Note that ``we show below that often, the weak limit of a first stage is supported in $\ell_{Lin,zero}^\infty(\mathcal{F}_c) \times \ell_{Lin,zero}^\infty(\mathcal{F}_c^c)$'', so the reader understands why we introduce it. \\
				
				Lemma \ref{Lemma: Hadamard differentiability, optimal transport, full differentiability} needs to be rewritten: if there is a unique Kantorovich potential, then $OT_{c,(P_1,P_0)}'$ is linear on $\big(\ell_{Lin,zero}^\infty(\mathcal{F}_c) \times \ell_{Lin,zero}^\infty(\mathcal{F}_c^c) \big) \cap \big(\mathcal{C}(\mathcal{F}_c, L_{2,P}) \times \mathcal{C}(\mathcal{F}_c^c, L_{2,P})\big)$.
				\begin{itemize}
					\item Here we run into a slight issue: the optimal transport literature says there's a unique KP if for every $(\varphi_1,\psi_1), (\varphi_2,\psi_2) \in \Psi(P_1,P_0)$, we have $\varphi_1 = \varphi_2 + c$, $P_1$-almost surely and $\psi_1 = \psi_2 - c$, $P_0$-almost surely. We use these almost-sure statements to claim that, when $(H_1, H_0) = (C_{1,P}'(\mathbb{G}), C_{0,P}'(\mathbb{G}))$ is an element of $\mathcal{C}(\mathcal{F}_c, L_{2,P_1}) \times \mathcal{C}(\mathcal{F}_c^c, L_{2,P_0})$, we can replace one with another: 
					\begin{equation*}
						H_1(\varphi_1) + H_0(\psi_1) = H_1(\varphi_2 - c) + H_0(\psi_2 + c) = H_1(\varphi_2) + H_0(\psi_2)
					\end{equation*}
					The first equality uses the almost-sure replacement, for which we required the continuity.
					 
					\item Now there's a subtle issue: for LATE, we only have a proof that $(H_1, H_0) = (C_{1,P}'(\mathbb{G}), C_{0,P}'(\mathbb{G}))$ is an element of $\mathcal{C}(\mathcal{F}_c, L_{2,P}) \times \mathcal{C}(\mathcal{F}_c^c, L_{2,P})$. Since this set is larger, we can't do the same replacement step if we only assume $\varphi_1 = \varphi_2 + c$, $P_1$-almost surely and $\psi_1 = \psi_2 - c$, $P_0$-almost surely. Since $L_{2,P}$ is stronger, some functions that are continuous wrt this semimetric may not be continuous wrt the weaker semimetrics $L_{2,P_1}$ and $L_{2,P_0}$. 
					
					\item Instead, we can write around this with the following: 
					\begin{enumerate}[label=(\alph*)]
						\item First, note that there are three notions of a unique KP with subtle differences.
						
						\item The first is what the optimal transport literature uses: a KP as unique in the original sense. Remark that when the KP is unique in this sense, the derivative is linear on $\mathcal{C}(\mathcal{F}_c, L_{2,P_1}) \times \mathcal{C}(\mathcal{F}_c^c, L_{2,P_0})$. Note that under exogenous treatment, $(C_{1,P}'(\mathbb{G}),  C_{0,P}'(\mathbb{G}))$ is an element of $\big(\ell_{Lin,zero}^\infty(\mathcal{F}_c) \times \ell_{Lin,zero}^\infty(\mathcal{F}_c^c) \big) \cap \big(\mathcal{C}(\mathcal{F}_c, L_{2,P_1}) \times \mathcal{C}(\mathcal{F}_c^c, L_{2,P_0})\big)$ (perhaps show the proof later?). 
						
						\item The second notion is enough for our purposes. Here's the formal lemma: if the KP is unique in the sense that for any $(\varphi_1,\psi_1), (\varphi_2,\psi_2) \in \Psi(P_1,P_0)$, we ahve $\varphi_1 = \varphi_2 + c$, $P$-almost surely and $\psi_1 = \psi_2 - c$, $P$-almost surely, then $OT_{c, (P_1,P_0)}'$ is linear on $\big(\ell_{Lin,zero}^\infty(\mathcal{F}_c) \times \ell_{Lin,zero}^\infty(\mathcal{F}_c^c) \big) \cap \big(\mathcal{C}(\mathcal{F}_c, L_{2,P}) \times \mathcal{C}(\mathcal{F}_c^c, L_{2,P})\big)$.
						
						\item Finally, the third and strongest notion: for any $(\varphi_1,\psi_1), (\varphi_2,\psi_2) \in \Psi(P_1,P_0)$, we have $\varphi_1(y_1) = \varphi_2(y_1) + c$ and $\psi_1(y_2) = \psi_2(y_2) - c$ for all $(y_1,y_2) \in \mathcal{Y}_1 \times \mathcal{Y}_2$. Follow this with the formal lemma \ref{Lemma: Kantorovich potential, sufficient conditions for uniqueness}, with the corrections noted below.
					\end{enumerate}
				\end{itemize}
				
				Lemma \ref{Lemma: Kantorovich potential, sufficient conditions for uniqueness} (sufficient conditions for a unique Kantorovich potential) can stay relatively unchanged.
				\begin{itemize}
					\item See \cite{staudt2022uniqueness} remark 1, theorem 2, and corollary 2 to fix the bit about the support.
					\item Their lemma 2 notes that $\text{Supp} \; \mu \setminus p_X(\text{supp} \; \pi)$ is a subset of $\Sigma$, which is defined later in equation (14) as ``the set of points $x \in \text{Supp} \; \mu$ such that $\pi$ does not \textit{induce regularity} at $x$.'' But since $Y$ is compact, we have that $\pi$ induces regularity on the whole of $\text{Supp} \; \mu$ (see the definition of regularity given in their equation (6)). So $\Sigma = \varnothing$.
					\item (For the above, we should probably just cite them... or just assert it without comment. The argument is complicated.) 
					\item Also note that their corollary 2 really does say the KP is unique at all points (up to the constant), even though they state it as ``almost surely''. To see this, note that the end of the proof of theorem 2 says $f_1 = f_2$ on $\text{Supp} \; \mu \setminus \Sigma$. As noted above, $\Sigma = \varnothing$.
				\end{itemize}
				
			\end{enumerate}
			
			\item Rewrite appendix \ref{Appendix: weak convergence}:
			\begin{enumerate}
				\item Introduce $C_{x_m} = (C_{1,x_m}, C_{0,x_m})$ for each case: exogenous treatment and LATE IV. Perhaps, to avoid confusion, have $C_{x_m}^{exo}$ and $C_{x_m}^{IV}$. 
				\item Write a lemma for Hadamard differentiability of $C_{d,x_m}$ for exogenous treatment and for LATE IV. Compare lemma \ref{Lemma: Hadamard differentiability, conditional distributions}. Write a quick corollary like \ref{Lemma: Hadamard differentiability, maps between bounded function spaces, corollary}.
				
				\item Cut lemma \ref{Lemma: weak convergence, conditional distributions} (thank god), as its no longer necessary.
				
				\item Replace lemma \ref{Lemma: weak convergence, conditional distributions, asymptotic distribution support} with a new lemma: 
				\begin{equation*}
					P\Big(C_{m,P}'(\mathbb{G}) \in \big(\ell_{Lin,zero}^\infty(\mathcal{F}_c) \times \ell_{Lin,zero}^\infty(\mathcal{F}_c^c) \big) \cap \big(\mathcal{C}(\mathcal{F}_c, L_{2,P}) \times \mathcal{C}(\mathcal{F}_c^c, L_{2,P})\big)\Big) = 1
				\end{equation*}
				This will be the most irritating...
				\begin{itemize}
					\item the proof of continuity is quick once we've shown the ``rearrangments'' are continuous in $L_{2,P}$. 
					\item The proof that the support is linear and evaluates constants to zero involves lots of calculation. But for now I don't see another way to do it.
				\end{itemize}
				
				\item Now a final lemma (that doesn't yet exist): The whole map, from $\ell^\infty(\mathcal{F}) \mapsto \sum_{x_m \in \mathcal{X}} P(X = x_m) OT_c(C_m(P))$, is Hadamard directionally differentiable at any $P$ such that 
			\end{enumerate}
		\end{enumerate}
	\end{mdframed}

	First note that in each possible setting, the distributions of interest are dominated by the unconditional distribution of the data with \textbf{bounded densities}.\footnote{
		\textbf{Question:} do we need that the density is bounded for the claim that $L_{2,P_d}(f_1, f_2) \leq A_d L_{2,P}(f_1,f_2)$? It's an unusual assumption to put into the lemma for differentiability of optimal transport. 
		
		Let $p > 0$. Since $f(y) = y^{\frac{p+1}{p}}$ is convex on $y \geq 0$, Jensen's inequality implies that 
		\begin{align*}
			E[\lvert X \rvert^{p+1}] = E[f(\lvert X \rvert^{p})] \geq f(E[\lvert X \rvert^p]) = (E[\lvert X \rvert^p])^{\frac{p+1}{p}}
		\end{align*}
		notice this implies $(E[\lvert X \rvert^{p+1}])^{1/(p+1)} \geq (E[\lvert X \rvert^p])^{1/p}$, and hence $L_{2,P}(f_1, f_2) \geq L_{2,P}(f_1, f_2)$ for any distribution $P$. 
		
		Now suppose $Q \ll P$. This implies 
		\begin{align*}
			L_{2,Q}(f_1, f_2) = \left(\int (f_1(x) - f_2(x))^2 \frac{dQ}{dP}(x) dP(x)\right)^{1/2} \geq \int \lvert f_1(x) - f_2(x)\rvert \frac{dQ}{dP}(x) dP(x) = L_{1,Q}(f_1, f_2)
		\end{align*}
		Meanwhile, a direct application of Jensen's with concavity of $g(x) = x^{1/2}$ for $x \geq 0$ implies
		\begin{align*}
			\left(\int (f_1(x) - f_2(x))^2 \frac{dQ}{dP}(x) dP(x)\right)^{1/2} \geq \int \lvert f_1(x) - f_2(x) \rvert \sqrt{\frac{dQ}{dP}(x)} dP(x)
		\end{align*}
		Hmmm.... this isn't giving me a lot to work with.

		For now I'll go ahead with the boundedness assumption, since it is satisfied.
	}
	\begin{itemize}
		\item For exogenous treatment, let $(Y,D) \sim P$, and note that $Y \mid D = 1 \sim P_1$ is the distribution of $Y_1$. $C_1$ is the transformation of $P \in \ell^\infty(\mathcal{F}_c)$:
		\begin{align*}
			E[\varphi(Y_1) \mid D = 1] = C_1(P)(\varphi) = \frac{E[\varphi(Y) D]}{P(D = 1)} = E\left[\varphi(Y) \frac{D}{P(D=1)}\right]
		\end{align*}
		But in particular, notice this implies $P$ dominates $P_1$ with density $\frac{dP_1}{dP}(y,d) = \frac{d}{P(D = 1)}(y,d)$. Similarly, if $P_0$ is the distribution of $Y_0$, we have $Y \mid D = 0 \sim P_0$ and $P_0$ has density $\frac{dP_0}{dP}(y,d) = \frac{1-d}{P(D=0)}$. With covariates, 
		\begin{align*}
			&\frac{dP_{1 \mid x_m}}{dP}(y, d, x_m) = \frac{d \times \mathbbm{1}\{X = x_m\}}{P(D = 1, X = x_m)}, &&\frac{dP_{0 \mid x_m}}{dP}(y, d, x_m) = \frac{(1-d) \times \mathbbm{1}\{X = x_m\}}{P(D = 0, X = x_m)}
		\end{align*}
		
		\item Next consider the LATE IV setting: $(Y, D, Z) \sim P$. Observe that 
		\begin{align*}
			E[\varphi(Y_1) \mid D_1 > D_0] &= C_1(P)(\varphi) = \frac{E[\varphi(Y)D \mid Z = 1] - E[\varphi(Y) D \mid Z = 0]}{P(D = 1 \mid Z = 1) - P(D = 1 \mid Z = 0)} \\
			&= \frac{E[\varphi(Y) DZ] / P(Z=1) - E[\varphi(Y) D(1-Z)]/P(Z = 0)}{P(D = 1, Z = 1)/P(Z = 1) - P(D = 1, Z = 0)/P(Z=0)} \\
			&= E\left[\varphi(Y) \frac{DZ/P(Z=1) - D(1-Z)/P(Z=0)}{P(D = 1, Z = 1)/P(Z = 1) - P(D = 1, Z = 0)/P(Z=0)}\right]
		\end{align*}
		shows that $P$ dominates $P_{1 \mid complier}$ with density $\frac{DZ/P(Z=1) - D(1-Z)/P(Z=0)}{P(D = 1, Z = 1)/P(Z = 1) - P(D = 1, Z = 0)/P(Z=0)}$. $P$ also dominates $P_{0 \mid complier}$, with a similar density. With covariates, the densities are only mildly more complicated with additional indicator functions and more probabilities.
	\end{itemize}
	
	\subsubsection{The outcome spaces}
	
	We're moving toward equipping $\mathcal{F}_c$ and $\mathcal{F}_c^c$ with $L_{2,P}$. To do so, the functions $\varphi$, $\psi$ need to be defined on the outcome space for $P$: 
	\begin{align*}
		&\varphi : \mathcal{Y} \rightarrow \mathbb{R}, &&\psi : \mathcal{Y} \rightarrow \mathbb{R}
	\end{align*}
	So we should start rewriting appendix \ref{Appendix: properties of optimal transport} to be titled \textbf{Properties of optimal transport on dominated distributions}. Make a small remark that some of these results apply more generally than conditional distributions, but they'll be applied here with conditional distributions.
	
	Begin this section by considering $P_1$ and $P_0$, distributions dominated by $P$ with bounded densities. Our two examples:
	\begin{enumerate}
		\item For exogenous treatment, we have $W = (Y,D,X) \sim P$, and $Y = D Y_1 + (1-D) Y_0$. Simply, $Y_d \sim P_d$. Densities: $\frac{dP_1}{dP}(d) = \frac{d}{P(D = 1)}$ and $\frac{dP_0}{dP}(d) = \frac{1-d}{P(D = 1)}$. 
		\item For endogenous treatment, $P_d$ is the distribution of $Y_d \mid D_1 > D_0$.
	\end{enumerate}
	View these distributions as $P_1,P_0 \in \mathcal{P}(\mathcal{Y})$, where $\mathcal{Y}$ is the outcome space of $Y = D Y_1 + (1-D)Y_0$. Note that we can work with $\mathcal{Y}$ equal to the union of the outcome spaces for $P_1$ and $P_0$. Next define the sets $\mathcal{F}_c$ and $\mathcal{F}_c^c$, for when $c$ is continuous or when $c$ is an indicator. Note they are just as discussed in the earlier appendix, but now defined on domains $\mathcal{Y}$. 
	
	Appendix \ref{Appendix: properties of optimal transport, subsection differentiability, subsubsection tangent set} is currently about the tangent set, but in the new version of things it'll be about completeness. Appendix \ref{Appendix: duality in optimal transport} contains lemmas \ref{Lemma: c-concave functions, smooth costs, completeness} and \ref{Lemma: c-concave functions, indicator of convex set costs, completeness}, which show that $\mathcal{F}_c$, $\mathcal{F}_c^c$, the product space $\mathcal{F}_c \times \mathcal{F}_c^c$, and the subset $\Phi_c \cap (\mathcal{F}_c \times \mathcal{F}_c^c)$  are complete. These will be moved here, and updated:
	\begin{itemize}
		\item Once we've shown $\mathcal{F}_c \times \mathcal{F}_c^c$ is complete, the argument there will imply $\varphi(y_1) + \psi(y_0) \leq c(y_1,y_0)$, $P$-almost surely. We need to argue it will hold for all points.
		\item The current argument assumes that $\mathcal{Y}_d = \text{Supp}(P_d)$, then uses continuity of $\varphi, \psi, c$. If we assume $\mathcal{Y} = \text{Supp}(P)$, I think the same argument goes through. So we can view $P_1,P_0 \in \mathcal{P}(\mathcal{Y})$, define $\varphi, \psi : \mathcal{Y} \rightarrow \mathbb{R}$, and simply assume that $\mathcal{Y} = \text{Supp}(Y)$. 
	\end{itemize}
	(The completeness lemma for indicator costs/$c$-concave functions, lemma \ref{Lemma: c-concave functions, indicator of convex set costs, completeness} works just fine as written, with the obvious adjustments.)

	\textbf{One may worry: does something potentially strange happen with instruments?}
	\begin{itemize}
		\item With instruments, we could define $\mathcal{Y}_d$ (if we define it at all) to be the outcome space of $Y_d \mid D_1 > D_0$. This is a subset of $\mathcal{Y}$, the outcome space of $Y$; to see it, first notice that 
		\begin{align*}
			Y &= D Y_1 + (1-D) Y_0 \\
			&= (ZD_1 + (1-Z)D_0)Y_1 + (1 - ((ZD_1 + (1-Z)D_0)))Y_0 \\
			&= (D_0 + Z(D_1 - D_0)) Y_1 + (1 - (D_0 + Z(D_1 - D_0)))Y_0 
		\end{align*}
		Now suppose $P(D_1 > D_0) > 0$. When $D_1 > D_0$, we have $D_1 = 1$ and $D_0 = 0$ and hence 
		\begin{align*}
			Y &= Z Y_1 + (1 - Z)Y_0
		\end{align*}
		(Aside: this observation is very cool. The subset of compliers behaves as though we're enforcing their treatment status.) 
		
		\item Since $Z$ is independent and non-degenerate, it's clear that any value of $Y_1$ or $Y_0$ possible when $D_1 > D_0$ is possible for $Y$. \textbf{So the outcome space of $Y_d \mid D_1 > D_0$ is a subset of the outcome space of $Y$.}
	\end{itemize}
	
	\textbf{The tough thing is organization.} Where should the completeness lemmas go?
	\begin{itemize}
		\item These lemmas are now not exactly general, but more specific to my context. It doesn't make as much sense to have them grouped in appendix \ref{Appendix: duality in optimal transport}, which summarizes well-known results from optimal transport.
		\item \textbf{I think they should be placed in appendix \ref{Appendix: properties of optimal transport, subsection differentiability}}, before showing differentiability. We can introduce the $L_2$ semimetric, then show it makes these sets complete, then show the general result and the corollary that applies it.
	\end{itemize}
	
	\subsubsection{Rewriting differentiability of optimal transport}
	
	Since these densities are bounded, we have that $L_{2,P}$ is stronger than $L_{2,P_d}$ for each $d = 0,1$. Say the bound is $A_d > 0$; i.e. $\frac{dP_d}{dP}(w) \leq A_d$. Then
	\begin{align*}
		L_{2,P_d}(f_1, f_2)^2 &= \int (f_1(w) - f_2(w))^2 dP_d(w) = \int (f_1(w) - f_2(w))^2 \frac{dP_d}{dP}(w) dP(w) \\
		&\leq A_d \int (f_1(w) - f_2(w))^2 dP(w) = A_d L_{2,P}(f_1, f_2)
	\end{align*}
	$L_{2,P_d}(f_1, f_2)^2 \leq A_d L_{2,P}(f_1,f_2)$ implies that $\mathcal{C}(\mathcal{F}_c, L_{2, P_d}) \subseteq \mathcal{C}(\mathcal{F}_c, L_{2, P})$. It's easy to see that $P_d \in \mathcal{C}(\mathcal{F}_c, L_{2, P_d})$ (see the proof of lemma \ref{Lemma: Hadamard differentiability, optimal transport}), so $P_d \in \mathcal{C}(\mathcal{F}_c, L_{2,P})$.
	
	\begin{mdframed}
		The above is enough to rewrite lemma \ref{Lemma: Hadamard differentiability, optimal transport} to the following: \\
		
		Suppose that $P$ dominates $P_1$ and $P_0$ with bounded densities, and that for some universally bounded $\mathcal{F}_c \subseteq L^1(P_1)$ and $\mathcal{F}_c^c \subseteq L^1(P_0)$, 
		\begin{enumerate}
			\item Strong duality holds:
			\begin{equation*}
				\inf_{\pi \in \Pi(P_1, P_0)} \int c(y_1, y_0) d\pi(y_1, y_0) = \sup_{(\varphi, \psi) \in \Phi_c \cap (\mathcal{F}_c \times \mathcal{F}_c^c)} \int \varphi(y_1) dP_1(y_1) + \int \psi(y_0) dP_0(y_0)
			\end{equation*}
			\item $\mathcal{F}_c$ and $\mathcal{F}_c^c$ are $P$-Donsker, and
			\item $(\mathcal{F}_c \times \mathcal{F}_c^c, L_2)$ and the subset
			\begin{equation*}
				\Phi_c \cap (\mathcal{F}_c \times \mathcal{F}_c^c) = \left\{(\varphi, \psi) \in \mathcal{F}_c \times \mathcal{F}_c^c \; ; \; \varphi(y_1) + \psi(y_0) \leq c(y_1, y_0)\right\}
			\end{equation*}
			are complete.
		\end{enumerate}
		Then $OT_c : \ell^\infty(\mathcal{F}_c) \times \ell^\infty(\mathcal{F}_c^c)$ defined by 
		\begin{align*}
			OT_c(P_1,P_0) = \sup_{(\varphi, \psi) \in \Phi_c \cap (\mathcal{F}_c \times \mathcal{F}_c^c)} P_1(\varphi) + P_0(\psi)
		\end{align*}
		is Hadamard directionally differentiable at $(P_1,P_0)$ tangentially to 
		\begin{equation*}
			\mathbb{D}_T = \mathcal{C}(\mathcal{F}_c, L_{2,P}) \times \mathcal{C}(\mathcal{F}_c^c, L_{2,P}) 
		\end{equation*}
		The set of maximizers $\Psi(P_1, P_0) = \argmax_{(\varphi, \psi) \in \Phi_c \cap (\mathcal{F}_c \times \mathcal{F}_c^c)} P_1(\varphi) + P_0(\psi)$ is nonempty, and the derivative $OT_{c,(P_1,P_0)}' : \mathbb{D}_0 \rightarrow \mathbb{R}$ is given by
		\begin{equation*}
			OT_{c, (P_1,P_0)}'(H_1, H_0) = \sup_{(\varphi, \psi) \in \Psi(P_1, P_0)} H_1(\varphi) + H_0(\varphi)
		\end{equation*}
	\end{mdframed}
	
	\subsubsection{The first stage: conditional distributions}
	
	To apply the delta method to claim weak convergence, we show that the transformation is Hadamard differentiable and the weak limit is supported in $\mathcal{C}(\mathcal{F}_c, L_{2,P}) \times \mathcal{C}(\mathcal{F}_c, L_{2,P})$. This step may be considerably more work. 
	
	Begin with $\mathcal{F}$, the relevant large Donsker set. Recall that $\sqrt{n}(\mathbb{P}_n - P) \overset{L}{\rightarrow} \mathbb{G}$ in $\ell^\infty(\mathcal{F})$ and, since $\mathcal{F}$ is universally bounded, $\mathbb{G}$ is supported in $\mathcal{C}(\mathcal{F}, L_{2,P})$.\footnote{\cite{vaart1997weak} example 1.5.10 shows that $\mathbb{G} \in \mathcal{C}(\mathcal{F}, \rho_2)$ with probability one, where $\rho_2$ is the intrinsic (variance) semimetric $\rho_2(f_1,f_2) = \sqrt{\text{Var}_P(f_1(W) - f_2(W))}$. Now simply note the $L_{2,P}$ semimetric is stronger than $\rho_2$; essentially the observations that $E[X^2] \geq \text{Var}(X)$.}
	
	Now observe that $C_1 : \ell^\infty(\mathcal{F}) \rightarrow \ell^\infty(\mathcal{F}_c)$ and $C_0 : \ell^\infty(\mathcal{F}) \rightarrow \ell^\infty(\mathcal{F}_c^c)$ are Hadamard differentiable at $P$, so $C : \ell^\infty(\mathcal{F}) \rightarrow \ell^\infty(\mathcal{F}_c) \times \ell^\infty(\mathcal{F}_c^c)$ is Hadamard differentiable at $P$ (see lemma \ref{Lemma: Hadamard differentiability, stacking functions}). The functional delta method (\cite{van2000asymptotic} lemma 20.8) implies that 
	\begin{align*}
		&\sqrt{n}(C(\mathbb{P}_n) - C(P)) \overset{L}{\rightarrow} C_{P}'(\mathbb{G}) \\
		\text{ equaivalently, } &\sqrt{n}((C_1(\mathbbm{P}_n), C_0(\mathbb{P}_n) - (C_1(P), C_0(P))) \overset{L}{\rightarrow} (C_{1,P}'(\mathbb{G}), C_{0,P}'(\mathbb{G}))
	\end{align*}
	
	Our goal is to show that 
	\begin{align*}
		P(C_P'(\mathbb{G}) \in \mathcal{C}(\mathcal{F}_c, L_{2,P}) \times \mathcal{C}(\mathcal{F}_c^c, L_{2,P})) = 1
	\end{align*}
	or equivalently,
	\begin{align*}
		P(C_{1,P}'(\mathbb{G}) \in \mathcal{C}(\mathcal{F}_c, L_{2,P}), C_{0,P}'(\mathbb{G}) \in \mathcal{C}(\mathcal{F}_c^c, L_{2,P})) = 1
	\end{align*}
	It suffices to show that $P(C_{1,P}'(\mathbb{G}) \in \mathcal{C}(\mathcal{F}_c, L_{2,P})) = 1$ and $P(C_{0,P}'(\mathbb{G}) \in \mathcal{C}(\mathcal{F}_c^c, L_{2,P})) = 1$ separately.\footnote{This follows the familiar fact: if $P(A) = 1$ and $P(B) = 1$, then $P(A \cap B) = 1$. Brief proof: recall $P(A \cap B) = P(A) + P(B) - P(A \cup B)$. Since $P(A \cup B) \geq P(B) = 1$, $(A \cap B) = 1 + 1 - 1 = 1$.}

	The following argument should work in each case: exogenous treatment or LATE IV, and to both $C_1$ and $C_0$. It is easier to explain with just one case. Consider $C_1$ in the LATE IV framework. This map consists of two parts: a ``rearrangement'', $R_1 : \ell^\infty(\mathcal{F}) \rightarrow \ell^\infty(\mathcal{F}_c)^K$, and composition with a function $q : \mathbb{R}^K \rightarrow \mathbb{R}$:
	\begin{equation*}
		C_1(g)(\varphi) = q(R_1(g)(\varphi))
	\end{equation*}
	The rearrangment is fully differentiable, and the arguments shown in lemma \ref{Lemma: Hadamard differentiability, conditional distributions} show that $q$ is fully differentiable at $R_1(P)$. As a result, $C_1$ is differentiable at $P$ and $C_{1,P}'$ resembles an inner product:
	\begin{align*}
		&C_{1,P}' : \ell^\infty(\mathcal{F}) \rightarrow \ell^\infty(\mathcal{F}_c), &&C_{1,P}'(g)(\varphi) = [\nabla q(R_1(P)(\varphi))]^\intercal R_1(g)(\varphi)
	\end{align*}
	where $\nabla q(R_1(P)(\varphi))$ and $R_1(g)(\varphi)$ are elements of $\mathbb{R}^K$. As a result,
	\begin{align*}
		C_{1,P}'(\mathbb{G})(\varphi) = \left[\nabla q(R_1(P)(\varphi))\right]^\intercal R_1(\mathbb{G})(\varphi)
	\end{align*}
	We can show $P(C_{1,P}'(\mathbb{G}) \in \mathcal{C}(\mathcal{F}_c, L_{2,P})) = 1$ in steps:
	\begin{enumerate}
		\item Show that $R_1(P)$ continuous with respect to $L_{2,P}$, and with probability one $R_1(\mathbb{G})$ is as well. We do so by showing that if $g \in \mathcal{C}(\mathcal{F}, L_{2,P})$, then $R_1(g)$ is continuous with respect to $L_{2,P}$.
		
		First recall that 
		\begin{align*}
			R_1(g)(\varphi) = (g(\mathbbm{1}_{1,1} \times \varphi), g(\mathbbm{1}_{1,1}), g(\mathbbm{1}_1), g(\mathbbm{1}_{1,0} \times \varphi), g(\mathbbm{1}_{1,0}), g(\mathbbm{1}_0))
		\end{align*}
		Now fix $\varphi$; we'll show $R_1(g)$ is continuous at $\varphi$. Note that for any $\tilde{\varphi}$,
		\begin{align*}
			R_1(g)(\varphi) - R_1(g)(\tilde{\varphi}) = (g(\mathbbm{1}_{1,1} \times \varphi) - g(\mathbbm{1}_{1,1} \times \tilde{\varphi}), 0, 0, g(\mathbbm{1}_{1,0} \times \varphi) - g(\mathbbm{1}_{1,0} \times \tilde{\varphi}), 0, 0)
		\end{align*}
		implying
		\begin{align*}
			\lVert R_1(g)(\varphi) - R_1(g)(\tilde{\varphi}) \rVert_2^2 &= \left[g(\mathbbm{1}_{1,1} \times \varphi) - g(\mathbbm{1}_{1,1} \times \tilde{\varphi})\right]^2 + \left[g(\mathbbm{1}_{1,0} \times \varphi) - g(\mathbbm{1}_{1,0} \times \tilde{\varphi})\right]^2
		\end{align*}
		Let $\varepsilon > 0$. Since $g \in \mathcal{C}(\mathcal{F}, L_{2,P})$, there exists $\delta_{1,1} > 0$ and $\delta_{1,0}$ such that 
		\begin{align*}
			L_{2,P}(\mathbbm{1}_{1,1} \times \varphi, \mathbbm{1}_{1,1} \times \tilde{\varphi})< \delta_{1,1} &\implies \lvert g(\mathbbm{1}_{1,1} \times \varphi) - g(\mathbbm{1}_{1,1} \times \tilde{\varphi})\rvert < \frac{\varepsilon}{\sqrt{2}} \\
			L_{2,P}(\mathbbm{1}_{1,0} \times \varphi, \mathbbm{1}_{1,0} \times \tilde{\varphi})< \delta_{1,0} &\implies \lvert g(\mathbbm{1}_{1,1} \times \varphi) - g(\mathbbm{1}_{1,1} \times \tilde{\varphi})\rvert < \frac{\varepsilon}{\sqrt{2}}
		\end{align*}
		Furthermore, notice that 
		\begin{align*}
			L_{2,P}(\mathbbm{1}_{1,1} \times \varphi, \mathbbm{1}_{1,1} \times \tilde{\varphi})^2 &= \int \mathbbm{1}_{1,1}(d,z) \times (\varphi(y) - \tilde{\varphi}(y))^2 dP(y,d,z) \\
			&\leq \int (\varphi(y) - \tilde{\varphi}(y))^2 dP(y,d,z) \\
			&= L_{2,P}(\varphi, \tilde{\varphi})^2
		\end{align*}
		and similarly, $L_{2,P}(\mathbbm{1}_{1,1} \times \varphi, \mathbbm{1}_{1,1} \times \tilde{\varphi}) \leq L_{2,P}(\varphi, \tilde{\varphi})$. Set $\delta = \max\{\delta_{1,1}, \delta_{1,0}\}$, and notice that $L_{2,P}(\varphi, \tilde{\varphi}) < \delta$ implies $L_{2,P}(\mathbbm{1}_{1,1} \times \varphi, \mathbbm{1}_{1,1} \times \tilde{\varphi})< \delta_{1,1}$ and $L_{2,P}(\mathbbm{1}_{1,0} \times \varphi, \mathbbm{1}_{1,0} \times \tilde{\varphi})< \delta_{1,0}$ and hence
		\begin{align*}
			\lVert R_1(g)(\varphi) - R_1(g)(\tilde{\varphi}) \rVert_2^2 &= \left[g(\mathbbm{1}_{1,1} \times \varphi) - g(\mathbbm{1}_{1,1} \times \tilde{\varphi})\right]^2 + \left[g(\mathbbm{1}_{1,0} \times \varphi) - g(\mathbbm{1}_{1,0} \times \tilde{\varphi})\right]^2 \\
			&< \left(\frac{\varepsilon}{\sqrt{2}}\right)^2 + \left(\frac{\varepsilon}{\sqrt{2}}\right)^2 = \varepsilon^2
		\end{align*}
		i.e. $\lVert R_1(g)(\varphi) - R_1(g)(\tilde{\varphi}) \rVert_2 < \varepsilon$. Thus $R_1(g)(\cdot)$ is continuous with respect to $L_{2,P}$.
		\begin{itemize}
			\item Now notice that since $P \in \mathcal{C}(\mathcal{F}, L_{2,P})$, we have $R_1(P) : \mathcal{F}_c \rightarrow \mathbb{R}^6$ is continuous with respect to $L_{2,P}$
			
			\item Recall that $P(\mathbb{G} \in \mathcal{C}(\mathcal{F}, L_{2,P})) = 1$, we have that $R_1(\mathbb{G}) : \mathcal{F}_c \rightarrow \mathbb{R}^6$ is continuous wrt $L_{2,P}$ with probability one as well. 
		\end{itemize}

		\item Since $q : \mathbb{D}_q \subseteq \mathbb{R}^6 \rightarrow \mathbb{R}$ is continuously differentiable, $\nabla q : \mathbb{D}_q \subseteq \mathbb{R}^6 \rightarrow \mathbb{R}^6$ is continuous. Since the composition of continuous functions is continuous, we have $\varphi \mapsto \nabla q(R_1(P)(\varphi))$ is continuous.
		
		\item Since $\langle \cdot, \cdot \rangle$ is continuous, $\varphi \mapsto \left[\nabla q(R_1(P)(\varphi))\right]^\intercal R_1(\mathbb{G})(\varphi) = \langle \nabla q(R_1(P)(\varphi)), R_1(\mathbb{G})(\varphi)\rangle$ is continuous with probability one.
	\end{enumerate}
	
	The same argument should work to show $C_{0,P}'(\mathbb{G}) \in \mathcal{C}(\mathcal{F}_c^c, L_{2,P})$ with probability one. I also believe the same argument should work for exogenous treatment.
	
	\subsubsection{Full differentiability on the support}
	
	Lemma \ref{Lemma: Hadamard differentiability, optimal transport, full differentiability} shows that if there is a unique Kantorovich potential and the support of the first stage is functions that are linear and evaluate constants to zero, then the derivative is linear on that support. 
	
	Before, we got there by working with $\mathcal{T}_{\mathcal{P}(\mathcal{Y}_d)}(P_d)$, which was easy because with exogenous treatment, $C_d(\mathbb{P}_n)$ is always probability distribution (i.e. $C_d(\mathbb{P}_n) \in \mathcal{P}(\mathcal{Y}_d)$). This is not so with the LATE IV identification; see \cite{kitagawa2015test}. 
	
	We'll take a different approach. For a set of real-valued functions $\mathcal{F}$, define
	\begin{align*}
		\ell_{Lin, zero}^\infty(\mathcal{F}) &= \Big\{g \in \ell^\infty(\mathcal{F}) \; ; \; \text{ for all } a, b\in \mathbb{R} \text{ and } f_1, f_2 \in \mathcal{F} \text{ such that } a f_1 + b f_2 \in \mathcal{F}, \\
		&\hspace{1 cm} g(a f_1 + b f_2) = a g(f_1) + b g(f_2), \text{ and if } a \in \mathcal{F}, \text{ then } g(a) = 0\Big\}
	\end{align*}
	It's easy to see that $\ell_{Lin,zero}^\infty(\mathcal{F})$ is closed: let $\{g_n\}_{n=1}^\infty \subseteq \ell_{Lin,zero}^\infty(\mathcal{F})$ be Cauchy and let $g$ be its limit in $\ell^\infty(\mathcal{F})$ (recall $\ell^\infty(\mathcal{F})$ is a Banach space). Note that this implies $0 = \lim_{n \rightarrow \infty} \lvert g_n(f) - g(f)\rvert$ for any function $f$, so
	\begin{align*}
		\left\lvert g_n(a f_1 + b f_2) - g(a f_1 + b f_2) \right\rvert = \left\lvert a g_n(f_1) + bg_n(f_2) - g(a f_1 + b f_2) \right\rvert 
	\end{align*}
	since $a g_n(f_1) + bg_n(f_2) \rightarrow a g(f_1) + b g(f_2)$ and limits are unique, we must have that $g$ is linear. Similarly, $0 = \lim_{n \rightarrow \infty}\lvert g_n(a) - g(a) \rvert = \lim_{n \rightarrow \infty}\lvert g(a) \rvert = \lvert g(a) \rvert$, so $g \in \ell_{Lin, zero}^\infty(\mathcal{F})$; therefore $\ell_{Lin,zero}^\infty(\mathcal{F})$ is closed. \\
	
	Now, follow a series of steps:
	\begin{enumerate}
		
		\item First notice that 
		\begin{align*}
			\sqrt{n}(\mathbb{P}_n(a) - P(a)) = \sqrt{n}(a - a) = 0
		\end{align*}
		and 
		\begin{align*}
			\sqrt{n}(\mathbb{P}_n(a f_1 + b f_2) - P(a f_1 + b f_2)) = a\sqrt{n}(\mathbb{P}_n(f_1) - P(f_2)) + b \sqrt{n}(\mathbb{P}_n(f_1) - P(f_2))
		\end{align*}
		and therefore $\sqrt{n}(\mathbb{P}_n - P) \in \ell_{Lin,zero}^\infty(\mathcal{F})$. \\
		
		Since $\ell_{Lin,zero}^\infty(\mathcal{F})$ is closed, Portmanteau shows that $\mathbb{G} \in \ell_{Lin,zero}^\infty(\mathcal{F})$ with probability one.
		
		\item Next we use this result to argue that $C_{1,P}'(\mathbb{G}) \in \ell_{Lin, zero}^\infty(\mathcal{F}_c)$. Recall that $C_{1,P}'(\mathbb{G})(\varphi) = [\nabla q(R_1(P)(\varphi))]^\intercal R_1(\mathbb{G}(\varphi))$. 
		\begin{itemize}
			\item Consider linearity first. Its not obvious $C_{1,P}'(\mathbb{G})(\varphi)$ is linear in $\varphi$; it appears quadratic. Through some manual calculations we can see that it is in fact linear.\footnote{I suspect what is needed here is that $q$ is linear in the ``expectation terms'', that is, for endogeneity $q(n_1, p_{11}, p_1, n_0, p_{10}, p_0) = \frac{n_1/p_1 - n_0/p_0}{p_{11}/p_1 - p_{10}/p_0} = \frac{n_1p_0 - n_0 p_1}{p_{11}p_0 - p_{10}p_1}$ is linear in $(n_1, n_0)$. Similarly, for exogenous treatment, $q(n,p) = \frac{n}{p}$ is linear in $n$.}

			First recall that
			\begin{align*}
				&q : \mathbb{D}_q \rightarrow \mathbb{R} &q(n_1, p_{11}, p_1, n_0, p_{10}, p_0) = \frac{n_1/p_1 - n_0/p_0}{p_{11}/p_1 - p_{10}/p_0} = \frac{n_1p_0 - n_0 p_1}{p_{11}p_0 - p_{10}p_1}
			\end{align*}
			and observe that $q$ is continuously differentiable on $\mathbb{D}_q$ with
			\begin{align*}
				&\nabla q(n_1, p_{11}, p_1, n_0, p_{10}, p_0) = 
				\begin{pmatrix}
					\frac{\partial q}{\partial n_1} & \frac{\partial q}{\partial p_{11}} & \frac{\partial q}{\partial p_1} & \frac{\partial q}{\partial n_0} & \frac{\partial q}{\partial p_{10}} & \frac{\partial q}{\partial p_0}
				\end{pmatrix} 
			\end{align*}
			where
			\begin{align*}
				&\frac{\partial q}{\partial n_1} = \frac{p_0}{p_{11}p_0 - p_{10}p_1} \\
				&\frac{\partial q}{\partial p_{11}} = -\frac{n_1p_0 - n_0 p_1}{(p_{11}p_0 - p_{10}p_1)^2} p_0 \\
				&\frac{\partial q}{\partial p_1} = \frac{(p_{11}p_0 - p_{10}p_1)(-n_0) - (n_1p_0 - n_0 p_1)(-p_{10})}{(p_{11}p_0 - p_{10}p_1)^2} \\
				& \frac{\partial q}{\partial n_0} = \frac{-p_1}{p_{11}p_0 - p_{10}p_1} \\
				& \frac{\partial q}{\partial p_{10}} = -\frac{n_1p_0 - n_0 p_1}{(p_{11}p_0 - p_{10}p_1)^2} (-p_1) \\
				& \frac{\partial q}{\partial p_0} = \frac{(p_{11}p_0 - p_{10} p_1)(n_1) - (n_1 p_0 - n_0 p_1)(p_{11})}{(p_{11}p_0 - p_{10} p_1)^2} 
			\end{align*}
			and since 
			\begin{align*}
				R_1(g)(\varphi) = (g(\mathbbm{1}_{1,1} \times \varphi), g(\mathbbm{1}_{1,1}), g(\mathbbm{1}_1), g(\mathbbm{1}_{1,0} \times \varphi), g(\mathbbm{1}_{1,0}), g(\mathbbm{1}_0))
			\end{align*}
			
			we have that 
			\begin{align*}
				&[\nabla q(R_1(P)(\varphi))]^\intercal R_1(\mathbb{G})(\varphi) \\
				&\hspace{1 cm} = \left[\frac{p_0}{p_{11}p_0 - p_{10}p_1}\right] \mathbbm{G}(\mathbbm{1}_{1,1} \times \varphi) + \left[-\frac{P(\mathbbm{1}_{1,1} \times \varphi) p_0 - P(\mathbbm{1}_{1,0} \times \varphi)  p_1}{(p_{11}p_0 - p_{10}p_1)^2} p_0\right]\mathbb{G}(\mathbbm{1}_{1,1}) \\
				&\hspace{1 cm} + \left[\frac{(p_{11}p_0 - p_{10}p_1)(-P(\mathbbm{1}_{1,0} \times \varphi)) - (P(\mathbbm{1}_{1,1} \times \varphi) p_0 - P(\mathbbm{1}_{1,0} \times \varphi) p_1)(-p_{10})}{(p_{11}p_0 - p_{10}p_1)^2}\right] \mathbbm{G}(\mathbbm{1}_1) \\
				&\hspace{1 cm} + \left[\frac{-p_1}{p_{11}p_0 - p_{10}p_1}\right]\mathbb{G}(\mathbbm{1}_{1,0} \times \varphi) + \left[-\frac{P(\mathbbm{1}_{1,1} \times \varphi) p_0 - P(\mathbbm{1}_{1,0} \times \varphi) p_1}{(p_{11}p_0 - p_{10}p_1)^2} (-p_1)\right]\mathbb{G}(\mathbbm{1}_{1,0}) \\
				&\hspace{1 cm} + \left[\frac{(p_{11}p_0 - p_{10} p_1)P(\mathbbm{1}_{1,1} \times \varphi) - (P(\mathbbm{1}_{1,1} \times \varphi) p_0 - P(\mathbbm{1}_{1,0} \times \varphi) p_1)(p_{11})}{(p_{11}p_0 - p_{10} p_1)^2} \right] \mathbb{G}(\mathbbm{1}_0)
			\end{align*}
			Examine each of the 6 terms in the RHS sum to see that 
			\begin{align*}
				&\left[\frac{p_0}{p_{11}p_0 - p_{10}p_1}\right] \mathbbm{G}(\mathbbm{1}_{1,1} \times (a \varphi_1 + b \varphi_2)) \\
				&\hspace{1 cm} = a\left[\frac{p_0}{p_{11}p_0 - p_{10}p_1}\right] \mathbbm{G}(\mathbbm{1}_{1,1} \times \varphi_1) + b\left[\frac{p_0}{p_{11}p_0 - p_{10}p_1}\right] \mathbbm{G}(\mathbbm{1}_{1,1} \times \varphi_2)
			\end{align*}
			and the other terms are similar: they are linear in $\varphi$. Thus
			\begin{align*}
				&[\nabla q(R_1(P)(a \varphi_1 + b \varphi_2))]^\intercal R_1(\mathbb{G})(a \varphi_1 + b \varphi_2) \\
				&\hspace{1 cm} = a[\nabla q(R_1(P)(\varphi_1))]^\intercal R_1(\mathbb{G})(\varphi_1) + b [\nabla q(R_1(P)(\varphi_2))]^\intercal R_1(\mathbb{G})(\varphi_2)
			\end{align*}
			i.e., $C_{1,P}'(\mathbb{G}) \in \ell^\infty(\mathcal{F}_c)$ is linear. 
			
			\item We can do a similarly manual observation that $C_{1,P}'(\mathbb{G})(a) = 0$ for constant functions $a$.\footnote{Here I'm not sure what property of $q$ is giving us this property of $C_{1,P}(\mathbb{G})(\cdot)$. I suspect it homogeneity of degree one in $(n_1,n_0)$? Regardless, it isn't as important \textit{why} it works if I can show that it does.}
			
			Specifically, consider the first two terms and notice that 
			\begin{align*}
				&\left[\frac{p_0}{p_{11}p_0 - p_{10}p_1}\right] \mathbbm{G}(\mathbbm{1}_{1,1} \times a) + \left[-\frac{P(\mathbbm{1}_{1,1} \times a) p_0 - P(\mathbbm{1}_{1,0} \times a)  p_1}{(p_{11}p_0 - p_{10}p_1)^2} p_0\right]\mathbb{G}(\mathbbm{1}_{1,1}) \\
				&\hspace{1 cm} = a \left[\frac{p_0}{p_{11}p_0 - p_{10}p_1}\right] \mathbbm{G}(\mathbbm{1}_{1,1}) + \left[-a \frac{P(\mathbbm{1}_{1,1}) p_0 - P(\mathbbm{1}_{1,0})  p_1}{(p_{11}p_0 - p_{10}p_1)^2}p_0\right] \mathbb{G}(\mathbbm{1}_{1,1})\\
				&\hspace{1 cm} = a \left[\frac{p_0}{p_{11}p_0 - p_{10}p_1}\right] \mathbbm{G}(\mathbbm{1}_{1,1}) -a \left[\frac{p_0}{p_{11}p_0 - P_{10}p_1}\right]\mathbb{G}(\mathbbm{1}_{1,1}) \\
				&\hspace{1 cm} = 0
			\end{align*}
			where the third equality uses $p_{11} = P(\mathbbm{1}_{1,1})$ and $p_{10} = P(\mathbbm{1}_{1,0})$. Consider the third term:
			\begin{align*}
				&\left[\frac{(p_{11}p_0 - p_{10}p_1)(-P(\mathbbm{1}_{1,0} \times a)) - (P(\mathbbm{1}_{1,1} \times a) p_0 - P(\mathbbm{1}_{1,0} \times a) p_1)(-p_{10})}{(p_{11}p_0 - p_{10}p_1)^2}\right] \mathbbm{G}(\mathbbm{1}_1) \\
				&\hspace{1 cm} = \left[\frac{a(p_{11}p_0 - p_{10}p_1)(-p_{10}) - a(p_{11}p_0 - p_{10}p_1)(-p_{10})}{(p_{11}p_0 - p_{10}p_1)^2}\right] \mathbb{G}(\mathbbm{1}_1) \\
				&\hspace{1 cm} = 0 \times \mathbb{G}(\mathbbm{1}_1)
			\end{align*}
			The fourth and fifth terms cancel similarly to the first and second, and the sixth is zero similar to the third. Thus $C_{1,P}'(\mathbb{G})(a) = 0$. 
		\end{itemize}

	\end{enumerate}
	
	\newpage

	\subsubsection{Support of LATE IV first stage THIS IS OLD, BUT MAY HAVE SOME CALCULATIONS I WANT TO USE/DOUBLE CHECK}
	
	Ignore covariates $X$ for now. As shown above, we have 
	\begin{align*}
		E[f(Y_1) \mid D_1 > D_0] &= \frac{E[f(Y)D \mid Z = 1] - E[f(Y) D \mid Z = 0]}{P(D = 1 \mid Z = 1) - P(D = 1 \mid Z = 0)}, \\
		& \\
		E[f(Y_0) \mid D_1 > D_0] &= \frac{E[f(Y)(1-D) \mid Z = 0] - E[f(Y) (1-D) \mid Z = 1]}{P(D = 0 \mid Z = 0) - P(D = 0 \mid Z = 1)} 
	\end{align*}
	
	Define 
	\begin{align*}
		&\mathbbm{1}_1(z) = \mathbbm{1}\{z = 1\}, &&\mathbbm{1}_0(z) = \mathbbm{1}\{z = 0\}
	\end{align*}
	and
	\begin{align*}
		&\mathbbm{1}_{1,1}(d,z) = \mathbbm{1}\{d = 1, z = 1\}, &\mathbbm{1}_{1,0}, \; \mathbbm{1}_{0,1}, \; \mathbbm{1}_{0,0}, \; \text{ similarly}
	\end{align*}
	The large Donsker set is
	\begin{align*}
		\mathcal{F} &= \left\{\mathbbm{1}_{1,1} \times \varphi \; ; \; \varphi \in \mathcal{F}_c\right\} \cup \left\{\mathbbm{1}_{1,0} \times \varphi \; ; \; \varphi \in \mathcal{F}_c\right\} \\
		&\hspace{1 cm} \cup \left\{\mathbbm{1}_{0,0} \times \psi \; ; \; \psi \in \mathcal{F}_c^c\right\} \cup \left\{\mathbbm{1}_{0,1} \times \psi \in \mathcal{F}_c^c\right\} \\
		&\hspace{1 cm} \cup \{\mathbbm{1}_1, \mathbbm{1}_0, \mathbbm{1}_{1,1}, \mathbbm{1}_{1,0}, \mathbbm{1}_{0,1}, \mathbbm{1}_{0,0}\}
	\end{align*}
	Now note that 
	\begin{align*}
		P_{1 \mid complier}(\varphi) = \frac{E[ \mathbbm{1}_{1,1}(D,Z)\varphi(Y)]/E[\mathbbm{1}_1(Z)] - E[\mathbbm{1}_{1,0}(D,Z)\varphi(Y)]/E[\mathbbm{1}_0(Z)]}{E[\mathbbm{1}_{1,1}(D,Z)]/E[\mathbbm{1}_1(Z)] - E[\mathbbm{1}_{1,0}(D,Z)]/E[\mathbbm{1}_0(Z)]}
	\end{align*}
	Is a map similar to the one studied in subsection \ref{Appendix: weak convergence, subsection conditional distributions}. Using similar arguments and notation to lemma \ref{Lemma: Hadamard differentiability, conditional distributions}, let $R_1$ map $\ell^\infty(\mathcal{F})$ to the appropriate product space of bounded functions, defined pointwise with
	\begin{align*}
		R_1(g)(\varphi) = (g(\mathbbm{1}_{1,1} \times \varphi), g(\mathbbm{1}_{1,1}), g(\mathbbm{1}_1), g(\mathbbm{1}_{1,0} \times \varphi), g(\mathbbm{1}_{1,0}), g(\mathbbm{1}_0))
	\end{align*}
	
	Next define $\mathbb{D}_q = \mathbb{R} \times (0,\infty) \times (0,\infty) \times \mathbb{R} \times (0,\infty) \times (0,\infty)$ and 
	\begin{align*}
		&q : \mathbb{D}_q \rightarrow \mathbb{R} &q(n_1, p_{11}, p_1, n_0, p_{10}, p_0) = \frac{n_1/p_1 - n_0/p_0}{p_{11}/p_1 - p_{10}/p_0} = \frac{n_1p_0 - n_0 p_1}{p_{11}p_0 - p_{10}p_1}
	\end{align*}
	
	and observe that $q$ is continuously differentiable on $\mathbb{D}_q$ with
	\begin{align*}
		&\nabla q(n_1, p_{11}, p_1, n_0, p_{10}, p_0) = 
		\begin{pmatrix}
			\frac{\partial q}{\partial n_1} & \frac{\partial q}{\partial p_{11}} & \frac{\partial q}{\partial p_1} & \frac{\partial q}{\partial n_0} & \frac{\partial q}{\partial p_{10}} & \frac{\partial q}{\partial p_0}
		\end{pmatrix}
	\end{align*}
	where
	\begin{align*}
		&\frac{\partial q}{\partial n_1} = \frac{p_0}{p_{11}p_0 - p_{10}p_1} \\
		&\frac{\partial q}{\partial p_{11}} = -\frac{n_1p_0 - n_0 p_1}{(p_{11}p_0 - p_{10}p_1)^2} p_0 = -\frac{\partial q}{\partial n_1}q \\
		&\frac{\partial q}{\partial p_1} = \frac{(p_{11}p_0 - p_{10}p_1)(-n_0) - (n_1p_0 - n_0 p_1)(-p_{10})}{(p_{11}p_0 - p_{10}p_1)^2} = \frac{p_{10} q - n_0}{p_{11}p_0 - p_{10}p_1} = \frac{\partial q}{\partial n_1} \frac{p_{10} q - n_0}{p_0} \\
		& \frac{\partial q}{\partial n_0} = \frac{-p_1}{p_{11}p_0 - p_{10}p_1} \\
		& \frac{\partial q}{\partial p_{10}} = -\frac{n_1p_0 - n_0 p_1}{(p_{11}p_0 - p_{10}p_1)^2} (-p_1) = -\frac{\partial q}{\partial n_0} q\\
		& \frac{\partial q}{\partial p_0} = \frac{(p_{11}p_0 - p_{10} p_1)(n_1) - (n_1 p_0 - n_0 p_1)(p_{11})}{(p_{11}p_0 - p_{10} p_1)^2} = \frac{-p_{11}q + n_1}{p_{11}p_0 - p_{10}p_1} = \frac{\partial q}{\partial n_0} \frac{p_{11}q - n_1}{p_1}
	\end{align*}

	The same arguments used in lemma \ref{Lemma: Hadamard differentiability, conditional distributions} work to show that 
	\begin{align*}
		&Q : \ell^\infty(\mathcal{F}) \rightarrow \ell^\infty(\mathcal{F}_c), &&Q(r)(\varphi) = q(r(\varphi))
	\end{align*}
	is fully differentiable at $R_1(P)$ tangentially to $\ell^\infty(\mathcal{F}_c)^6$ with derivative $Q_{R_1(g)}' : \ell^\infty(\mathcal{F}_c)^6 \rightarrow \ell^\infty(\mathcal{F}_c)$ given pointwise by 
	\begin{align*}
		Q_{R_1(g)}'(r)(\varphi) = \left[\nabla q(R_1(g)(\varphi))\right]^\intercal r(\varphi) 
	\end{align*}
	Thus the chain rule implies $C_1 : \ell^\infty(\mathcal{F}) \rightarrow \ell^\infty(\mathcal{F}_c)$ given by
	\begin{align*}
		C_1(g)(\varphi) = Q(R_1(g))(\varphi) = q(R_1(g)(\varphi))
	\end{align*}
	is fully Hadamard differentiable at $P$ tangentially to $\ell^\infty(\mathcal{F})$ with derivative 
	\begin{align*}
		C_{1,P}'(h)(\varphi) = \left[\nabla q(R_1(P)(\varphi))\right]^\intercal R_1(h)(\varphi) 
	\end{align*}
	
	The delta method step is similar to lemma \ref{Lemma: weak convergence, conditional distributions}, but with a much more tedious calculation of the covariance function. Since $\sqrt{n}(\mathbb{P}_n - P) \overset{L}{\rightarrow} \mathbb{G}$ in $\ell^\infty(\mathcal{F})$, The delta method implies 
	\begin{align*}
		&\sqrt{n}(C_1(\mathbb{P}_n) - C_1(P)) \overset{L}{\rightarrow} C_{1,P}'(\mathbb{G}) &&\text{ in } \ell^\infty(\mathcal{F}_c)
	\end{align*}
	where $C_{1,P}'(\mathbb{G})$ is mean-zero and Gaussian. Notice that 
	\begin{align*}
		C_{1,P}'(\mathbb{G})(\varphi) &= \left[\nabla q(R_1(P)(\varphi))\right]^\intercal R_1(\mathbb{G})(\varphi) 
	\end{align*}
	
	It follows that the covariance function of $C_{1,P}'(\mathbb{G})$ is given by
	\begin{align*}
		&\text{Cov}(\varphi_1, \varphi_2) = E[C_{1,P}'(\mathbb{G})(\varphi_1)C_{1,P}'(\mathbb{G})(\varphi_2)] \\
		&\hspace{1 cm} = E\left[\left[\nabla q(R_1(P)(\varphi_1))\right]^\intercal R_1(\mathbb{G})(\varphi_1)[R_1(\mathbb{G})(\varphi_2)]^\intercal \left[\nabla q(R_1(P)(\varphi_2))\right]\right] \\
		&\hspace{1 cm} = \left[\nabla q(R_1(P)(\varphi_1))\right]^\intercal E\left[R_1(\mathbb{G})(\varphi_1)[R_1(\mathbb{G})(\varphi_2)]^\intercal \right]\left[\nabla q(R_1(P)(\varphi_2))\right]
	\end{align*}
	
	To save notation, define
	\begin{align*}
		&E_{1,1,12} = E_P[\mathbbm{1}_{1,1} \varphi_1 \varphi_2] &&E_{1,1,1} = E_P[\mathbbm{1}_{1,1} \varphi_1] &&E_{1,1,2} = E_P[\mathbbm{1}_{1,1} \varphi_2] \\
		&E_{1,0,12} = E_P[\mathbbm{1}_{1,0} \varphi_1 \varphi_2]  &&E_{1,0,1} = E_P[\mathbbm{1}_{1,0} \varphi_1] &&E_{1,0,2} = E_P[\mathbbm{1}_{1,0} \varphi_2] \\
		&p_{1,1} = E_P[\mathbbm{1}_{1,1}] &&p_{1,0} = E[\mathbbm{1}_{1,0}], &&p_1 = E_P[\mathbbm{1}_1] && p_0 = E_P[\mathbbm{1}_0]
	\end{align*}
	Since $P_{1 \mid c}(\varphi) \coloneqq P_{1 \mid complier}(\varphi) = q(R_1(P)(\varphi))$, we have
	\begin{align*}
		R_1(\mathbb{G})(\varphi) &= 
		\begin{pmatrix}
			\mathbb{G}(\mathbbm{1}_{1,1} \times \varphi), \mathbb{G}(\mathbbm{1}_{1,1}), \mathbb{G}(\mathbbm{1}_1), \mathbb{G}(\mathbbm{1}_{1,0} \times \varphi), \mathbb{G}(\mathbbm{1}_{1,0}), \mathbb{G}(\mathbbm{1}_0)
		\end{pmatrix}^\intercal \\
		\nabla q(R_1(P)(\varphi_1)) &= 
		\begin{pmatrix}
			\frac{\partial q}{\partial n_1} & \frac{\partial q}{\partial p_{11}} & \frac{\partial q}{\partial p_1} & \frac{\partial q}{\partial n_0} & \frac{\partial q}{\partial p_{10}} & \frac{\partial q}{\partial p_0} 
		\end{pmatrix}^\intercal \\
		&= 
		\begin{pmatrix}
			\frac{p_0}{p_{1,1}p_0 - p_{1,0}p_1} & -\frac{\partial q}{\partial n_1}q_1 & \frac{\partial q}{\partial n_1} \frac{p_{1,0} q_1 - E_{1,0,1}}{p_0} & \frac{-p_1}{p_{1,1}p_0 - p_{1,0}p_1} & -\frac{\partial q}{\partial n_0} q_1 & \frac{\partial q}{\partial n_0} \frac{p_{1,1}q_1 - E_{1,1,1}}{p_1}
		\end{pmatrix}
	\end{align*}
	where recall $\frac{\partial q}{\partial n_1} = \frac{p_0}{p_{1,1}p_0 - p_{1,0}p_1}$ and $\frac{\partial q}{\partial n_0} = \frac{-p_1}{p_{1,1}p_0 - p_{1,0}p_1}$.
	
	\begin{landscape}
		
		The inner expectation is the following $6 \times 6$ matrix. First notice that $\mathbbm{1}_{1,1} \mathbbm{1}_0 = \mathbbm{1}\{D = 1, Z = 1\}\mathbbm{1}\{Z = 0\} = 0$, and similarly $\mathbbm{1}_{1,0} \mathbbm{1}_1 = \mathbbm{1}_1 \mathbbm{1}_0 = \mathbbm{1}_{1,1} \mathbbm{1}_{1,0} = 0$, etc.
		\begin{align*}
			&E\left[R_1(\mathbb{G})(\varphi_1)[R_1(\mathbb{G})(\varphi_2)]^\intercal \right] \\
			&\hspace{1 cm} = 
			\begin{bmatrix}
				\text{Cov}(\mathbbm{1}_{1,1} \varphi_1, \mathbbm{1}_{1,1} \varphi_2) & \text{Cov}(\mathbbm{1}_{1,1} \varphi_1, \mathbbm{1}_{1,1}) & \text{Cov}(\mathbbm{1}_{1,1} \varphi_1, \mathbbm{1}_1) & \text{Cov}(\mathbbm{1}_{1,1} \varphi_1, \mathbbm{1}_{1,0} \varphi_2) & \text{Cov}(\mathbbm{1}_{1,1} \varphi_1, \mathbbm{1}_{1,0}) & \text{Cov}(\mathbbm{1}_{1,1} \varphi_1, \mathbbm{1}_0) \\
				\text{Cov}(\mathbbm{1}_{1,1}, \mathbbm{1}_{1,1} \varphi_2) & \text{Cov}(\mathbbm{1}_{1,1}, \mathbbm{1}_{1,1}) &  \text{Cov}(\mathbbm{1}_{1,1}, \mathbbm{1}_1) & \text{Cov}(\mathbbm{1}_{1,1}, \mathbbm{1}_{1,0} \varphi_2) & \text{Cov}(\mathbbm{1}_{1,1}, \mathbbm{1}_{1,0}) & \text{Cov}(\mathbbm{1}_{1,1}, \mathbbm{1}_0) \\
				\text{Cov}(\mathbbm{1}_1, \mathbbm{1}_{1,1} \varphi_2) & \text{Cov}(\mathbbm{1}_1, \mathbbm{1}_{1,1}) & \text{Cov}(\mathbbm{1}_1, \mathbbm{1}_1) & \text{Cov}(\mathbbm{1}_1, \mathbbm{1}_{1,0} \varphi_2) & \text{Cov}(\mathbbm{1}_1, \mathbbm{1}_{1,0}) & \text{Cov}(\mathbbm{1}_1, \mathbbm{1}_0) \\
				\text{Cov}(\mathbbm{1}_{1,0} \varphi_1, \mathbbm{1}_{1,1} \varphi_2) & \text{Cov}(\mathbbm{1}_{1,0} \varphi_1, \mathbbm{1}_{1,1}) & \text{Cov}(\mathbbm{1}_{1,0} \varphi_1, \mathbbm{1}_1) & \text{Cov}(\mathbbm{1}_{1,0} \varphi_1, \mathbbm{1}_{1,0} \varphi_2) & \text{Cov}(\mathbbm{1}_{1,0} \varphi_1, \mathbbm{1}_{1,0}) & \text{Cov}(\mathbbm{1}_{1,0} \varphi_1, \mathbbm{1}_0) \\
				\text{Cov}(\mathbbm{1}_{1,0}, \mathbbm{1}_{1,1} \varphi_2) & \text{Cov}(\mathbbm{1}_{1,0}, \mathbbm{1}_{1,1}) & \text{Cov}(\mathbbm{1}_{1,0}, \mathbbm{1}_1) & \text{Cov}(\mathbbm{1}_{1,0}, \mathbbm{1}_{1,0} \varphi_2) & \text{Cov}(\mathbbm{1}_{1,0}, \mathbbm{1}_{1,0}) & \text{Cov}(\mathbbm{1}_{1,0}, \mathbbm{1}_0) \\
				\text{Cov}(\mathbbm{1}_0, \mathbbm{1}_{1,1} \varphi_2) & \text{Cov}(\mathbbm{1}_0, \mathbbm{1}_{1,1}) & \text{Cov}(\mathbbm{1}_0, \mathbbm{1}_1) &  \text{Cov}(\mathbbm{1}_0, \mathbbm{1}_{1,0} \varphi_2) & \text{Cov}(\mathbbm{1}_0, \mathbbm{1}_{1,0}) & \text{Cov}(\mathbbm{1}_0, \mathbbm{1}_0) \\
			\end{bmatrix} \\
			&\hspace{1 cm} = 
			\begin{bmatrix}
				E_{1,1,12} - E_{1,1,1} E_{1,1,2} & E_{1,1,1}(1 - p_{1,1}) & E_{1,1,1}(1 - p_1) & -E_{1,1,1}E_{1,0,2} & -E_{1,1,1}p_{1,0} & -E_{1,1,1}p_0 \\
				E_{1,1,2}(1 - p_{1,1}) & p_{1,1}(1-p_{1,1}) &  p_{1,1}(1 - p_1) & -p_{1,1} E_{1,0,2} & -p_{1,1}p_{1,0} & -p_{1,1}p_0 \\
				E_{1,1,2}(1 - p_1) & p_{1,1}(1-p_1) & p_1(1-p_1) & -p_1 E_{1,0,2}& -p_1p_{1,0} & -p_1 p_0 \\
				-E_{1,0,1}E_{1,1,2} & -E_{1,0,1}p_{1,1} & -E_{1,0,1}p_1 & E_{1,0,12} - E_{1,0,1}E_{1,0,2} & E_{1,0,1}(1-p_{1,0}) & E_{1,0,1}(1-p_0) \\
				-p_{1,0}E_{1,1,2} & -p_{1,0}p_{1,1} & -p_{1,0}p_1 & E_{1,0,2}(1-p_{1,0}) & p_{1,0}(1-p_{1,0}) & p_{1,0}(1-p_0) \\
				-p_0E_{1,1,2} & -p_0 p_{1,1} & -p_0 p_1 &  E_{1,0,2}(1-p_0) & p_{1,0}(1-p_0) & p_0(1-p_0) \\
			\end{bmatrix}
		\end{align*}
		Finally, we can compute the covariance function: 
		\begin{align*}
			&\text{Cov}(\varphi_1, \varphi_2) = E[C_{1,P}'(\mathbb{G})(\varphi_1)C_{1,P}'(\mathbb{G})(\varphi_2)] \\
			&\hspace{1 cm} = \left[\nabla q(R_1(P)(\varphi_1))\right]^\intercal E\left[R_1(\mathbb{G})(\varphi_1)[R_1(\mathbb{G})(\varphi_2)]^\intercal \right]\left[\nabla q(R_1(P)(\varphi_2))\right] \\
			&\hspace{1 cm} = 
		\end{align*}
		
		\begin{mdframed}
			The MATLAB code \verb|ComputeCovarianceMatrix_LATEIV.m| computes this symbolically - but as I suspected, the result is a mess. I'm unsure whether there's a mistake (in the on-paper calculations or putting it into MATLAB), but it's not at all obvious from the result whether the corresponding result is supported in $\mathcal{C}(\mathcal{F}_c, L_{2, P_{1 \mid complier}})$. 
		\end{mdframed}
	\end{landscape}

	\newpage

\end{singlespace}
