# Supplementary material for: Estimating Functionals of the Joint Distribution of Potential Outcomes with Optimal Transport
Source: arXiv:2311.09435 source file (2023-11-15)
Supplement: Supplementary file 3 [file OTJointPO_appendix_notation.tex]

\section{(CUT) Notation and Assumptions}

\begin{singlespace}
	This section won't appear in the final paper; it's just here to make the appendix easy to write.
	
	\subsection{Notation}
	
	\begin{itemize}
		\item Sample: $\{Y_i, D_i, X_i\}_{i=1}^n$, i.i.d.
		\begin{itemize}
			\item Observed and potential outcomes $Y_i = D_i Y_{1i} + (1-D_i)Y_{0i}\in \mathbb{R}$
			\item Treatment status: $D_i \in \{0,1\}$ 
			\item Covariates: $X_i \in \mathcal{X} = \{x_1, \ldots, x_M\} \subseteq \mathbb{R}^{d_x}$
		\end{itemize}
		\item Unconfoundedness: $(Y_1, Y_0)$ is jointly independent of $D$ conditional on covariates:
		\begin{equation*}
			(Y_1, Y_0) \perp D \mid X = x
		\end{equation*}
		Note that this is implied by the stronger assumption $(Y(1), Y(0), X) \perp D_i$\footnote{Sketch:
			\begin{align*}
				P(D = d, (Y(1), Y(0)) \in A\mid X = x) &= P(D = d \mid(Y(1), Y(0)) \in A,  X = x)P((Y(1), Y(0)) \in A \mid X = x) \\
				&= P(D = d \mid X = x)P((Y(1), Y(0)) \in A \mid X = x)
			\end{align*}
		}
		
		\item Joint and marginal distributions: 
		\begin{align*}
			&(Y_1, Y_0, X) \sim P, &&(Y_1, Y_0) \sim P_{1,0}, &&Y_d \sim P_d, \\
			&p_{dx} = P(D = d, X = x), &&p_x = P(X = x), &&p_d = P(D = d)
		\end{align*}
		
		\item Conditional distributions (and their support):
		\begin{align*}
			&Y_d \mid X = x \sim P_{d \mid x}, &&\mathcal{Y}_{d \mid x} = \text{Supp}(Y_d \mid X = x)
		\end{align*}
		
		\item Identified information: 
		\begin{align*}
			&P_{d \mid x} &&\text{and } &&p_{dx} = P(D = d, X = x) &&\text{ for all } (d,x) \in \{0,1\} \times \mathcal{X}.
		\end{align*}
		Notice that if we had the copula for $Y(1), Y(0)$ for each $x$, we could construct $P$.
		
		\item For $\Omega \subseteq \mathbb{R}^d$, let $\mathcal{P}(\Omega)$ denote the set of probability distributions on $\Omega$ (equipped with standard Borel sigma algebra).
		
		\item Set of joint distributions with given marginals:
		\begin{equation*}
			\Pi(P_{1 \mid x}, P_{0 \mid x}) = \left\{\pi \in \mathcal{P}(\mathcal{Y}_{1\mid x} \times \mathcal{Y}_{0 \mid x}) \; ; \; \pi_{1 \mid x} = P_{1 \mid x}, \; \pi_{0 \mid x} = P_{0 \mid x}\right\}
		\end{equation*}
		
		\item Nuisance parameters:
		\begin{align*}
			&\theta_0 = E[c(Y_1, Y_0)], &&\eta_0 = E\left[\begin{pmatrix} \eta_1(Y_1) \\ \eta_0(Y_0)\end{pmatrix} \right] \in \mathbb{R}^{d_\eta}
		\end{align*}
		where $c(y_1,y_0)$ is a function of both potential outcomes, and $\eta_d(y_d)$ is a function of only one potential outcome.
		
		\item Parameter of interest: $\gamma_0 \in \mathbb{R}$. Several cases:
		\begin{enumerate}[label=(\roman*)]
			\item $\gamma_0 = g(\theta_0, \eta_0)$, or 
			\item $\gamma_0$ is the $\tau$-th quantile of $Y(1) - Y(0)$.
		\end{enumerate} 
		Notice a special case of the first is $\gamma_0 = \theta_0$. Remark: the identified set of  $\theta_0$ implies the identified set for $\gamma_0$; we focus on identified set of $\theta_0$.
		
		\item Identified set of $\theta_0$ is $\Theta_I \subseteq \mathbb{R}$. 
		\begin{itemize}
			\item Notice $\theta_0 = E[E[c(Y_1, Y_0) \mid X]] = \sum_x p_x E[c(Y_1, Y_0) \mid X = x]$. Let $\Theta_I(x)$ be the identified set for $\theta(x) = E[c(Y_1, Y_0) \mid X = x]$, and notice that 
			\begin{align*}
				\Theta_I(x) &= \left\{\theta \in \Theta \; ; \; \theta = E_{\pi_x}[c(Y_1, Y_0)] \text{ where } \pi_x \in \Pi(P_{1 \mid x}, P_{0 \mid x}) \right\} \\
				\Theta_I &= \left\{\theta \in \Theta \; ; \; \theta = \sum_x p_x E_{\pi_x}[c(Y_1, Y_0)] \text{ where } \pi_x \in \Pi(P_{1 \mid x}, P_{0 \mid x}) \text{ for each } x \in \mathcal{X}\right\}
			\end{align*}
			Notice $\Theta_I(x)$ and $\Theta_I$ are convex, becuase $\Pi(P_{1 \mid x}, P_{0 \mid x})$ is convex. 
			
			\item Let $\theta_0(x) = E[c(Y_1, Y_0) \mid X = x]$. The identified set $\Theta_I(x) \subseteq \mathbb{R}$ is also convex.
		\end{itemize}
		
		\item Optimal transport with (lower semicontinuous) cost function $c$:
		\begin{equation*}
			OT_c(P_{1 \mid x}, P_{0 \mid x}) = \inf_{\pi \in \Pi(P_{1 \mid x}, P_{0 \mid x})} E_\pi[c(Y_1, Y_0)]
		\end{equation*}
		
		\item Bounds on $\theta_0(x)$:
		\begin{itemize}
			\item if $c$ is continuous,
			\begin{align*}
				&\theta^L(x) = OT_c(P_{1 \mid x}, P_{0 \mid x}), &&\theta^H(x) = -OT_{-c}(P_{1 \mid x}, P_{0 \mid x})
			\end{align*}
			
			\item if $c(y_1,y_0) = \mathbbm{1}\{y_1 - y_0 \leq \delta\}$, 
			\begin{align*}
				&c_L(y_1, y_0) = \mathbbm{1}\{y_1 - y_0 < \delta\}, &&c_H(y_1, y_0) = \mathbbm{1}\{y_1 - y_0 > \delta\}, \\
				&\theta^L(x) = OT_{c_L}(P_{1 \mid x}, P_{0 \mid x}), &&\theta^H(x) = 1 - OT_{c_H}(P_{1 \mid x}, P_{0 \mid x})
			\end{align*}
		\end{itemize}
		either way, define bounds on $\theta_0$:
		\begin{align*}
			&\theta^L = E[\theta^L(X)] = \sum_{x \in \mathcal{X}} p_x \theta^L(x), &&\theta^H = E[\theta^H(X)] =  \sum_{x \in \mathcal{X}} p_x \theta^H(x)
		\end{align*}

		\item Under assumption \ref{Assumption: setting} and \ref{Assumption: parameter, function of moments}, we have that $[\theta^L(x), \theta^H(x)]$ is the sharp identified set for $\theta_0(x)$. 
		\begin{itemize}
			\item When $c(y_1,y_0)$ is continuous, this is because \cite{villani2009optimal} theorem 4.1 shows optimal transport is attained 
			\item When $c(y_1, y_0) = \mathbbm{1}\{y_1 - y_0 \leq \delta\}$, this is because $\theta^H(x)$ is attained for each $x$. $\theta^L(x)$ can be shown sharp under the additional assumption that one of the distributions is continuously distributed
			\begin{itemize}
				\item \cite{fan2010sharp} never defines the distribution function, but cites 
			\end{itemize}
		\end{itemize}

		\item Remark: lesser bounds on $\theta_0$: 
		\begin{itemize}
			\item if $c$ is continuous,
			\begin{align*}
				&\tilde{\theta}^L = OT_c(P_1, P_0), &&\tilde{\theta}^H = -OT_{-c}(P_1, P_0)
			\end{align*}
			\item if $c(y_1,y_0) = \mathbbm{1}\{y_1 - y_0 \leq \delta\}$, 
			\begin{align*}
				&c_L(y_1, y_0) = \mathbbm{1}\{y_1 - y_0 < \delta\}, &&c_H(y_1, y_0) = \mathbbm{1}\{y_1 - y_0 > \delta\}, \\
				&\tilde{\theta}^L = OT_{c_L}(P_1, P_{0 \mid x}), &&\tilde{\theta}^H = 1 - OT_{c_H}(P_{1 \mid x}, P_{0 \mid x})
			\end{align*}
		\end{itemize}
		\cite{villani2009optimal} theorem 4.8 shows that $\tilde{\theta}^L \leq \theta^L$ and $\theta^H \leq \tilde{\theta}^H$; i.e. the bounds found by ignoring covariate information are larger.

		\item Denote the identified set for $\gamma_0$ as $\Gamma_I \subseteq \mathbb{R}$.
		
		\item Bounds on $\gamma_0$ when $\gamma_0 = g(\theta_0, \eta_0)$:
		\begin{align*}
			&\gamma^L = \inf_{\theta \in [\theta^L, \theta^H]} g(\theta, \eta_0) &&\gamma^H = \sup_{\theta \in [\theta^L, \theta^H]} g(\theta, \eta_0)
		\end{align*}
		\begin{itemize}
			\item $[\theta^L, \theta^H]$ is compact under assumption \ref{Assumption: parameter, function of moments}. So these problems are attained, and hence $\Gamma_I = [\gamma^L, \gamma^H]$, by continuity of $g(\cdot,\eta_0)$ and the intermediate value theorem.
		\end{itemize}

		\item Bounds on $\gamma_0$, the $\tau$-th quantile of $Y(1) - Y(0)$. Recall that 
		\begin{align*}
			&\gamma_0 = \inf\{t \; ; \; F_{Y_1 - Y_0}(t) \geq \tau\}, &&F_{Y_1 - Y_0}(t) = P(Y_1 - Y_0 \leq t)
		\end{align*}
		Define
		\begin{align*}
			&c_{L, \gamma}(y_1, y_0) = \mathbbm{1}\{y_1 - y_0 < \gamma\}, &&c_{H, \gamma}(y_1, y_0) = \mathbbm{1}\{y_1 - y_0 > \gamma\}, \\
			&F^L(\gamma \mid x) = OT_{c_{L, \gamma}}(P_{1 \mid x}, P_{0 \mid x}), &&F^H(\gamma \mid x) = 1 - OT_{c_{H, \gamma}}(P_{1 \mid x}, P_{0 \mid x}), \\
			&F^L(\gamma) = \sum_x p_x F^L(\gamma \mid x) &&F^H(\gamma) = \sum_x p_x F^H(\gamma \mid x)
		\end{align*}
		\textbf{Conjecture/claim:} If $\gamma \in \Gamma_I$ then $F^L(\gamma) \leq \tau \leq F^H(\gamma)$. Further suppose $F^L$ and $F^H$ are strictly increasing. Then $\gamma \in \Gamma_I$ if and only if $F^L(\gamma) \leq \tau \leq F^H(\gamma)$
		\begin{itemize}
			\item We can construct a confidence set for $\gamma_0$ by inverting a hypothesis test of 
			\begin{equation*}
				H_\gamma : F^L(\gamma) \leq \tau \leq F^H(\gamma) 
			\end{equation*}
			against the alternative $H_\gamma$ is not true.
		\end{itemize}
		
	\end{itemize}
\end{singlespace}

\subsection{Assumptions}

\assumptionSetting*
%\assumptionParameter*
%\assumptionCDF*
\assumptionCostFunction*
\assumptionParameterFunctionOfMoments*
