# Supplementary material for: Estimating Functionals of the Joint Distribution of Potential Outcomes with Optimal Transport
Source: arXiv:2311.09435 source file (2023-11-15)
Supplement: Supplementary file 4 [file OTJointPO_appendix_orthogonal_score.tex]

\section{Orthogonal Score}

\begin{mdframed}
	It would be great to have an orthogonal score for $(\theta^L, \theta^H)$ (or $(\gamma^L, \gamma^H)$). 
	
	I suspect this is possible, at least under the assumptions of lemma \ref{Lemma: Kantorovich potential, sufficient conditions for uniqueness}. This implies the Kantorovich potential is unique up to constant shifts (for all values in the domain, not just almost-surely). 
	
	If this doesn't work out (or, more likely, the deadline kills it) then I'll dump this whole section.
\end{mdframed}

\subsection{Influence function}

\begin{mdframed}
	\textbf{Note:} I think this is correct. But Andres notes that the thing to do is simply provide an orthogonal score - I don't need to prove that it was based on the influence function. 
	
	A better approach is simply to guess and check. He says this sounds like a perfectly reasonable guess; it's essentially just the envelope theorem (and recentering so the function has mean zero).
	
	Wrap this into the other functions to get a complete guess, then verify. 
\end{mdframed}

Lemma \ref{Lemma: Kantorovich potential, sufficient conditions for uniqueness} implies a very strong version of uniqueness of the Kantorovich potential: for any $(\varphi_1,\psi_1), (\varphi_2,\psi_2) \in \Psi(P_1,P_0)$, $\varphi_1^{cc} - \varphi_2^{cc}$ is a constant for \textit{all} values $y_1 \in \mathcal{Y}_1$ (not just $P_1$-almost all).

Suppose the conditions of lemma \ref{Lemma: Kantorovich potential, sufficient conditions for uniqueness} hold true, and let $(\varphi^*, \psi^*)$ denote this solution. Let $(P_{1t}, P_{0t}) = (P_1, P_0) + t\big((\tilde{P}_1, \tilde{P}_0) - (P_1, P_0)\big)$. Then I claim that 
\begin{align*}
	\lim_{t \downarrow 0} \frac{OT_c(P_{1t}, P_{0t}) - OT_c(P_1, P_0)}{t} &= \int \varphi^*(y_1) (d\tilde{P}_1 - dP_1) - \int \varphi^{*c}(y_0) (d\tilde{P}_1 - dP_0) \\
	&= \int \varphi^*(y_1) d\tilde{P}_1 + \int \psi^*(y_0) d\tilde{P}_0(y_0) - OT_c(P_1, P_0)
\end{align*}

\begin{proof}
	\singlespacing
	
	(SKETCH)
	
	We closely follow the proof of \cite{santambrogio2015optimal} proposition 7.17.
	
	Let $t_n \downarrow 0$ with $t_n \neq 0$. It suffices to show 
	\begin{equation*}
		\lim_{n \rightarrow \infty} \frac{OT_c(P_{1t_n}, P_{0t_n}) - OT_c(P_1, P_0)}{t_n} = \int \varphi^*(y_1) (d\tilde{P}_1 - dP_1) - \int \varphi^{*c}(y_0) (d\tilde{P}_1 - dP_0)
	\end{equation*}

	To see that the $\liminf$ is above the claimed limit, begin by noting that since $(\varphi^*, \psi^*)$ is optimal for $(P_1, P_0)$ but not necessarily optimal for $(P_{1t_n}, P_{0t_n})$,
	\begin{align*}
		&\frac{OT_c(P_{1t_n}, P_{0t_n}) - OT_c(P_1, P_0)}{t_n} \\
		&\hspace{1 cm} \geq \frac{\int \varphi^*(y_1) dP_{1t_n}(y_1) + \int \psi^*(y_0) dP_{0t_n}(y_0) - \int \varphi^*(y_1) dP_1(y_1) - \int \psi^*(y_0) dP_0(y_0)}{t_n} \\
		&\hspace{1 cm} = \int \varphi^*(y_1) (d\tilde{P}_1 - dP_1) - \int \psi^*(y_0) (d\tilde{P}_1 - dP_0) 
	\end{align*}
	implying that
	\begin{align*}
		\liminf_{n \rightarrow \infty} \frac{OT_c(P_{1t_n}, P_{0t_n}) - OT_c(P_1, P_0)}{t_n} \geq \int \varphi^*(y_1) (d\tilde{P}_1 - dP_1) - \int \psi^*(y_0) (d\tilde{P}_1 - dP_0) 
	\end{align*}
	
	Now consider the $\limsup_{n \rightarrow \infty} \frac{OT_c(P_{1t_n}, P_{0t_n}) - OT_c(P_1, P_0)}{t_n}$. Choose a subsequence $t_{n_k}$ realizing the $\limsup$:
	\begin{equation*}
		\lim_{k \rightarrow \infty} \frac{OT_c(P_{1t_{n_k}}, P_{0t_{n_k}}) - OT_c(P_1, P_0)}{t_{n_k}} = \limsup_{n \rightarrow \infty} \frac{OT_c(P_{1t_n}, P_{0t_n}) - OT_c(P_1, P_0)}{t_n}
	\end{equation*}
	Since $c$ is bounded on $\mathcal{Y}_1 \times \mathcal{Y}_0$, \cite{villani2009optimal} theorem 5.10 implies there exists a dual solution $(\varphi_k^*, \psi_k^*)$ for $(P_{1t_{n_k}}, P_{0t_{n_k}})$. Since $(\varphi_k^*, \psi_k^*)$ is optimal for $(P_{1t_{n_k}}, P_{0t_{n_k}})$ but not necessarily optimal for $(P_1, P_0)$,
	\begin{align*}
		&\frac{OT_c(P_{1t_{n_k}}, P_{0t_{n_k}}) - OT_c(P_1, P_0)}{t_{n_k}} \\
		&\hspace{1 cm} \leq \frac{\int \varphi_k^*(y_1) dP_{1t_{n_k}}(y_1) + \int \psi_k^*(y_0) dP_{0t_{n_k}}(y_0) - \int \varphi_k^*(y_1) dP_1(y_1) - \int \psi_k^*(y_0) dP_0(y_0)}{t} \\
		&\hspace{1 cm} = \int \varphi_k^*(y_1) (d\tilde{P}_1 - dP_1) - \int \psi_k^*(y_0) (d\tilde{P}_1 - dP_0) 
	\end{align*}
	
	$(\varphi_k^*, \psi_k^*)$ are elements of $\mathcal{F}_c \times \mathcal{F}_c^c$ with $\mathcal{F}_c$ and $\mathcal{F}_c^c$ defined by \eqref{Defn: F_c for smooth costs} and \eqref{Defn: F_c^c for smooth costs} respectively. The sequences $(\varphi_k^*, \psi_k^*)$ are thus uniformly bounded and uniformly equicontinuous. Their domains are the compact $\mathcal{Y}_1$ and $\mathcal{Y}_0$ respectively. Arzeli Ascoli (theorem 7.25 in Rudin's Principles of Mathematical Analysis) implies there exists a uniformly convergent subsequence $\{(\varphi_{k_j}^*, \psi_{k_j}^{*c})\}$. Let $(\tilde{\varphi}, \tilde{\psi})$ be that uniform limit. Since all elements of $\mathcal{F}_c$ and $\mathcal{F}_c^c$ are uniformly bounded, the dominated convergence theorem implies that 
	\begin{align*}
		\lim_{k \rightarrow \infty} \int \varphi_k^*(y_1) (d\tilde{P}_1 - dP_1) - \int \psi_k^*(y_0) (d\tilde{P}_1 - dP_0) &= \lim_{j \rightarrow \infty} \int \varphi_{k_j}^*(y_1) (d\tilde{P}_1 - dP_1) - \int \psi_{k_j}^*(y_0) (d\tilde{P}_1 - dP_0) \\
		&= \int \tilde{\varphi}(y_1) (d\tilde{P}_1 - dP_1) - \int \tilde{\psi}(y_0) (d\tilde{P}_1 - dP_0) 
	\end{align*}
	In summary, we have shown
	\begin{align*}
		\limsup_{n \rightarrow \infty} \frac{OT_c(P_{1t_n}, P_{0t_n}) - OT_c(P_1, P_0)}{t_n} &= \lim_{k \rightarrow \infty} \frac{OT_c(P_{1t_{n_k}}, P_{0t_{n_k}}) - OT_c(P_1, P_0)}{t_{n_k}} \\
		&= \int \tilde{\varphi}(y_1) (d\tilde{P}_1 - dP_1) - \int \tilde{\psi}(y_0) (d\tilde{P}_1 - dP_0) 
	\end{align*}
	
	The next goal is to show $(\tilde{\varphi}, \tilde{\psi})$ is optimal for $(P_1, P_0)$, which implies $(\tilde{\varphi}, \tilde{\psi}) = (\varphi^*, \psi^*) + (s, -s)$ for some constant $s \in \mathbb{R}$ (for every value $(y_1, y_0) \in \mathcal{Y}_1 \times \mathcal{Y}_0$) by uniqueness. This implies
	\begin{align*}
		\int \tilde{\varphi}(y_1) (d\tilde{P}_1 - dP_1) - \int \tilde{\psi}(y_0) (d\tilde{P}_1 - dP_0)  &= \int \varphi(y_1) + s(d\tilde{P}_1 - dP_1) - \int \psi(y_0) - s (d\tilde{P}_1 - dP_0) \\
		&= \int \varphi(y_1)(d\tilde{P}_1 - dP_1) - \int \psi(y_0)(d\tilde{P}_1 - dP_0) 
	\end{align*}
	and will complete the proof.
	
	Note that $\varphi_{k_j}^*(y_1) + \psi_{k_j}^*(y_0) \leq c(y_1, y_0)$ implies that $\tilde{\varphi}(y_1) + \tilde{\psi}(y_0) \leq c(y_1, y_0)$ and hence $(\tilde{\varphi}, \tilde{\psi})$ is feasible for the dual problem with $(P_1, P_0)$. Furthermore, $(P_{1t_n}, P_{0t_n}) \rightarrow (P_1, P_0)$ in $\ell^\infty(\mathcal{F}_c) \times \ell^\infty(\mathcal{F}_c^c)$:
	\begin{align*}
		\left\lVert (P_{1t_n}, P_{0t_n}) - (P_1, P_0) \right\rVert_\infty &= \left\lVert (P_{1t_n}, P_{0t_n}) - (P_1, P_0) \right\rVert_\infty \\
		&= \left\lVert (P_1, P_0) + t_n\big((\tilde{P}_1, \tilde{P}_0) - (P_1, P_0)\big) - (P_1, P_0)\right\rVert_\infty \\
		&= t_n \left\lVert (\tilde{P}_1, \tilde{P}_0) \right\rVert_\infty
	\end{align*}
	and since $OT_c$ is continuous (lemma \ref{Lemma: optimal transport is continuous}, $OT_c(P_{1t_n}, P_{0t_n}) \rightarrow OT_c(P_1, P_0)$, and hence  $OT_c(P_{1t_{n_{k_j}}}, P_{0t_{n_{k_j}}}) \rightarrow OT_c(P_1, P_0)$.
	
	The final thing to show is 
	\begin{align*}
		\int \varphi_{k_j}(y_1) dP_{1t_{n_{k_j}}}(y_1) + \int \varphi_{k_j}(y_0) dP_{1t_{n_{k_j}}}(y_0) \rightarrow \int \tilde{\varphi}(y_1) dP_1(y_1) + \int \tilde{\varphi}(y_0) dP_1(y_0)
	\end{align*}
	Since the LHS is $OT_c(P_{1t_{n_{k_j}}}, P_{0t_{n_{k_j}}})$, which has limit $OT_c(P_1,P_0)$, this will imply the desired
	\begin{equation*}
		OT_c(P_1, P_0) = \int \tilde{\varphi}(y_1) dP_1(y_1) + \int \tilde{\varphi}(y_0) dP_1(y_0)
	\end{equation*}
	
	It's clearly enough to show $\int \varphi_{k_j}(y_1) dP_{1t_{n_{k_j}}}(y_1) \rightarrow \int \tilde{\varphi}(y_1) dP_1(y_1)$ and similarly for hte other component. This is equivalently phrased as $\lvert P_{1t_{n_{k_j}}}(\varphi_{k_j}) - P_1(\tilde{\varphi}) \rvert \rightarrow 0$. Notice that 
	\begin{align*}
		\lvert P_{1t_{n_{k_j}}}(\varphi_{k_j}) - P_1(\tilde{\varphi}) \rvert  \leq \lvert P_{1t_{n_{k_j}}}(\varphi_{k_j}) - P_1(\varphi_{k_j}) \rvert + \lvert P_1(\varphi_{k_j}) - P_1(\tilde{\varphi}) \rvert
	\end{align*}
	Now use $P_{1t_{n_{k_j}}} \rightarrow P_1$ in $\ell^\infty(\mathcal{F}_c)$ to see the first has limit zero, and $P_1(\cdot)$ being continuous wrt $\mathcal{C}(\mathcal{F}_c, \lVert \cdot\rVert_\infty)$ to see the second has limit zero. This completes (a sketch of) the proof.
\end{proof}
