# Supplementary material for: Estimating Functionals of the Joint Distribution of Potential Outcomes with Optimal Transport
Source: arXiv:2311.09435 source file (2023-11-15)
Supplement: Supplementary file 5 [file OTJointPO_appendix_parameters.tex]

\section{(CLEAN) Parameters of interest}

\begin{enumerate}
	\item $\text{Cov}(Y_1, Y_0) = E[Y_1 Y_0] - E[Y_1]E[Y_0]$. 
	
	\item $\text{Corr}(Y_1, Y_0) = \frac{\text{Cov}(Y_1, Y_0)}{\sqrt{\text{Var}(Y_1)}\sqrt{\text{Var}(Y_0)}}$
	
	\item $\text{Var}(Y_1 - Y_0) = E[(Y_1 - Y_0)^2] - (E[Y_1] - E[Y_0])^2$
	
	\item $\text{Cov}(Y_1 - Y_0, Y_0) = E[(Y_1 - Y_0)Y_0] - (E[Y_1] - E[Y_0])E[Y_0]$
	\begin{itemize}
		\item If negative, units with $Y_0$ below $E[Y_0]$ tend to see $Y_1 - Y_0$ above $E[Y_1 - Y_0]$. 
	\end{itemize}
	
	\item $\text{Corr}(Y_1 - Y_0, Y_0) = \frac{\text{Cov}(Y_1 - Y_0, Y_0)}{\sqrt{\text{Var}(Y_1 - Y_0)}\sqrt{\text{Var}(Y_0)}} = \frac{\text{Cov}(Y_1, Y_0) - \text{Var}(Y_0)}{\sqrt{\text{Var}(Y_1) + \text{Var}(Y_0) - 2\text{Cov}(Y_1,Y_0)}\sqrt{\text{Var}(Y_0)}}$
	\begin{itemize}
		\item Same motivation as $\text{Cov}(Y_1 - Y_0, Y_0)$, but unitless.
		\item Appears non-monotonic in $\text{Cov}(Y_1,Y_0)$ when $\text{Var}(Y_0) > \text{Var}(Y_1)$; see \href{https://www.desmos.com/calculator/9puo7lzlrb}{this Desmos graph.}
	\end{itemize}

	\item $E\left[\frac{Y_1 - Y_0}{Y_0}\right] = E\left[\frac{Y_1}{Y_0}\right] - 1$. 
	\begin{itemize}
		\item The expected percent difference in $Y$. Useful if $Y_0$ has considerable range; if the outcome is yearly income, $Y_1 - Y_0 = \$5,000$ isn't much for $Y_0 = \$100,000$, but is quite nice if $Y_0 = \$30,000$. 
	\end{itemize}

	\item The $k$-th coefficient in the linear regression 
	\begin{align*}
		&Y_1 = \beta Y_0 + Z'\gamma + \varepsilon, &&E\left[\begin{pmatrix} Y_0 \\ Z \end{pmatrix}\varepsilon \right] = 0 
	\end{align*}
	\begin{itemize}
		\item $\gamma = e_k' \left(E\begin{bmatrix} Y_0^2 & Y_0 Z' \\ Z Y_0 & ZZ' \end{bmatrix}\right)^{-1} E\begin{bmatrix} Y_0 Y_1 \\ Z Y_1\end{bmatrix}$ where $Z \in \mathbb{R}^{d_z}$ and the sample is $\{Y_i, D_i, X_i, Z_i\}_{i=1}^n$
		\item Here $\theta = E[Y_1Y_0]$. Note that $g$ is monotonic in $\theta$, but the direction of the monotonicity depends on the (identified) first coordinate of $e_k'E\begin{bmatrix} Y_0^2 & Y_0 Z' \\ Z Y_0 & ZZ' \end{bmatrix}^{-1}$. 
		\item IV models are similar.
	\end{itemize}

	\item $E[u(Y_1 - Y_0)]$ for known utility function $u(\cdot)$. 

	\item $\sqrt{\text{Var}(Y_1 - Y_0)}/E[Y_1 - Y_0]$
	\begin{itemize}
		\item This is the ``coefficient of variation'' of $Y_1 - Y_0$, a less popular measure of inequality suggested by \cite{fan2017partial}.
	\end{itemize}

	\item $E[Y_1 - Y_0] / \sqrt{\text{Var}(Y_1 - Y_0)}$.
	\begin{itemize}
		\item Essentially a ``studentized'' treatment effect.
	\end{itemize}
	
	\item $P(Y_1 - Y_0 > \delta)$ for known $\delta$
	\begin{itemize}
		\item Especially, $P(Y_1 - Y_0 > \text{cost})$
	\end{itemize}
	
	\item The $\tau$-th quantile of $Y_1 - Y_0$; but we instead work with $\gamma$ solving 
	\begin{equation*}
		P(Y_1 - Y_0 \leq \gamma) = \tau
	\end{equation*}
	See section \ref{Section: extensions, subsection quantiles}.
\end{enumerate}

\subsection{Motivating discussion}

\begin{itemize}
	\item Consider the following risk analysis for treating $m$ i.i.d. units (e.g., establishments) at a known fixed cost. Without treatment unit $j$ returns $Y_{0j}$, with treatment $Y_{1j}$. The decision to be made is to treat all $m$ units or none of them. Treating all $m$ units is profitable if $\frac{1}{m} \sum_{j=1}^m Y_{1j} - Y_{0j} > \text{cost}$. 
	
	If we knew $\text{Var}(Y_1 - Y_0)$, then we have
	\begin{align*}
		\text{Var}\left(\frac{1}{m} \sum_{j=1}^m Y_{1j} - Y_{0j}\right) = \frac{1}{m} \text{Var}(Y_1 - Y_0)
	\end{align*}

	If we further assume $Y_1 - Y_0$ is normally distributed, then we can estimate the probability $\frac{1}{m} \sum_{j=1}^m Y_{1j} - Y_{0j} > \text{cost}$; i.e. the probability the venture is profitable:
	\begin{align*}
		P\left(\frac{1}{m} \sum_{j=1}^m Y_{1j} - Y_{0j} > \text{cost}\right) &= P\left(\frac{\frac{1}{m} \sum_{j=1}^m Y_{1j} - Y_{0j} - \text{ATE}}{\sqrt{\frac{1}{m} \text{Var}(Y_1 - Y_0)}} > \frac{\text{cost} - \text{ATE}}{\sqrt{\frac{1}{m} \text{Var}(Y_1 - Y_0)}}\right) \\
		&= \Phi\left(\sqrt{m}\frac{(\text{cost} - \text{ATE})}{\sqrt{\text{Var}(Y_1 - Y_0)}}\right)
	\end{align*}
	and if $m$ is large, the central limit theorem implies this approximates the probability of interest.

	\item Consider an RCT with multiple treatment arms: $Y = \sum_k D_k Y_k$. When $E[Y_1 - Y_0] \approx E[Y_2 - Y_0]$, it may be worth while to compare the treatments along other dimensions. For example, policy makers may prefer treatment $k$ with larger $P(Y_k - Y_0 > \text{cost}_k)$. 
	\begin{itemize}
		\item The identified set is a rectangle formed of the individual identified sets, because of the gluing lemma (\cite{villani2009optimal} p. 11).
	\end{itemize}
\end{itemize}
