# Supplementary material for: Estimating Functionals of the Joint Distribution of Potential Outcomes with Optimal Transport
Source: arXiv:2311.09435 source file (2023-11-15)
Supplement: Supplementary file 6 [file OTJointPO_appendix_identification_OLD_7Sept2023.tex]

\section{Identification}
\label{Appendix: identification}

\subsection{Identification Lemmas}
\label{Appendix: identification, subsection lemmas}

\begin{restatable}[]{lemma}{lemmaLATEIVMarginalDistributionIdentification}
	\label{Lemma: identification, LATE IV marginal distribution identification}
	
	UNFINISHED: PROVE THAT IN THE LATE IV SETTING,
	\begin{align*}
		E[f(Y_1) \mid D_1 > D_0, X = x] &= \frac{E[f(Y) D \mid X = x, Z = 1] - E[f(Y) D \mid X = x, Z = 0]}{P(D = 1 \mid X = x, Z = 1) - P(D = 1 \mid X = x, Z = 0)} \\
		E[f(Y_0) \mid D_1 > D_0, X = x] &= \frac{E[f(Y) (1-D) \mid X = x, Z = 0] - E[f(Y) (1-D)\mid X = x, Z = 1]}{P(D = 0 \mid X = x, Z = 0) - P(D = 0 \mid X = x, Z = 1)}
	\end{align*}
	
\end{restatable}
\begin{proof}
	UNFINISHED
\end{proof}

\begin{restatable}[]{lemma}{lemmaDegenerateImpliesSingletonCoupling}
	\label{Lemma: identification, degenerate distribution has only one coupling}
	\singlespacing
	
	Let $P_1$ be any distribution and $P_0$ be degenerate at $\tilde{y}_0 \in \mathbb{R}$. Then the only possible coupling of $P_1$ and $P_0$ is characterized by the cumulative distribution function
	\begin{align*}
		P(Y_1 \leq y_1, Y_0 \leq y_0) = \begin{cases}
			P(Y_1 \leq y_1) &\text{ if } y_0 \geq \tilde{y}_0 \\
			0 &\text{ if } y_0 < \tilde{y}_0
		\end{cases}
	\end{align*}
\end{restatable}
\begin{proof}
	\singlespacing
	
	First suppose $y_0 < \tilde{y}_0$. Then $0 \leq P(Y_1 \leq y_1, Y_0 \leq y_0) \leq P(Y_0 \leq y_0) = 0$.

	Next suppose $y_0 \geq \tilde{y}_0$. Then $1 \geq P(\{Y_1 \leq y_1\} \cup \{Y_0 \leq y_0\}) \geq P(Y_0 \leq y_0) = 1$ implies that 
	\begin{align*}
		P(Y_1 \leq y_1, Y_0 \leq y_0) &= P(Y_1 \leq y_1) + \underbrace{P(Y_0 \leq y_0)}_{=1} - \underbrace{P(\{Y_1 \leq y_1\} \cup \{Y_0 \leq y_0\})}_{=1} \\
		& = P(Y_1 \leq y_1)
	\end{align*}
	which completes the proof.
\end{proof}

\lemmaIdentificationFunctionOfMoments*
\begin{proof}
	\singlespacing
	
	In steps:
	
	\begin{enumerate}
		\item The identified set of the distribution of the primitives $(Y_1, Y_0, D, X)$ is characterized by $\pi_{1, 0 \mid x} \in \Pi(P_{1 \mid x}, P_{0 \mid x})$ for each $x$. 
		
		To see this claim, note that the i.i.d. sample $\{Y_i, D_i, X_i\}_{i=1}^n$ identifies $p_{dx} = P(D = d, X = x)$ and the conditional distributions of $Y$ given $D = d, X = x$. Assumption \ref{Assumption: setting} \ref{Assumption: setting, RCT/unconfoundedness} is $(Y_1, Y_0) \perp D \mid X$, which implies
		\begin{align*}
			&Y \mid D = 1, X = x \sim P_{1 \mid x} &&Y \mid D = 0, X = x \sim P_{0 \mid x}
		\end{align*}
		where $Y_d \mid X = x$ for each $d = 0,1$. Thus the identified information is $P_{1\mid x}$ ,$P_{0 \mid x}$, and $p_{dx}$. 
		
		Note that for any measurable set $A$,
		\begin{align*}
			P((Y_1, Y_0) \in A, D = d, X = x) &= P((Y_1, Y_0) \in A \mid X = x) P(D = d, X = x)
		\end{align*}
		Examine the right hand side, and note that specifying $\pi_x \in \Pi(P_{1 \mid x}, P_{0 \mid x})$ for each $x$ completes the distribution of $(Y_1, Y_0, D, X)$. Furthermore, any such set of $\pi_x$ is consistent with the identified information and assumption \ref{Assumption: setting}. 
		
		\item The identified set for $\theta$, denoted $\Theta_I$, is convex.
		
		Note that for any $\theta \in \Theta_I$, there exists a distribution $\pi$ over the primitives $(Y_1, Y_0, D, X)$ characterized by $\pi_x \in \Pi(P_{1 \mid x}, P_{0 \mid x})$. So for any $\theta, \tilde{\theta} \in \Theta_I$ and any $\lambda \in (0,1)$, there exists $\pi_x, \tilde{\pi}_x \in \Pi(P_{1 \mid x}, P_{0 \mid x})$ such that $\theta = \int E_{\pi_x}[c(Y_1, Y_0)] dP_X(x)$ and $\tilde{\theta} = \int E_{\tilde{\pi}_x}[c(Y_1, Y_0)] dP_X(x)$, thus
		\begin{equation*}
			\lambda \theta + (1-\lambda) \tilde{\theta} =\int \lambda E_{\pi_{1, 0 \mid x}}[c(Y_1, Y_0)] + (1-\lambda)E_{\tilde{\pi}_{1, 0 \mid x}}[c(Y_1, Y_0)] dP_X(x)
		\end{equation*}
		Since $\Pi(P_{1 \mid x}, P_{0 \mid x})$ (defined in \eqref{Defn: Pi, distributions with given marginals}) is a convex set, $\lambda \pi_{1, 0 \mid x} + (1-\lambda)\tilde{\pi}_{1, 0 \mid x} \in \Pi(P_{1 \mid x}, P_{0 \mid x})$ characterizes a distribution $\pi^\lambda$ over $(Y_1, Y_0, D, X)$, which rationalizes $\theta^\lambda = \lambda \theta + (1-\lambda)\tilde{\theta}$. Thus $\Theta_I$ is convex. 
		
		\item We next argue $\Theta_I = [\theta^L, \theta^H]$. Moreover, $\theta^L$ and $\theta^H$ are finite.
		
		Assumption \ref{Assumption: parameter, function of moments} \ref{Assumption: parameter, function of moments, cost function, Lipschitz} and the extreme value theorem implies $c$ is bounded on $\mathcal{Y}_1 \times \mathcal{Y}_0$. Optimal transport with lower semicontinuous costs that are bounded from below is attained (see lemma \ref{Lemma: optimal transport is attained}), so there exists $\pi_x^L, \pi_x^H \in \Pi(P_{1 \mid x}, P_{0 \mid x})$ such that 
		\begin{align*}
			&E_{\pi_x^L}[c(Y_1, Y_0)] = \theta^L(x) = \inf_{\pi_x \in \Pi(P_{1 \mid x}, P_{0 \mid x})} E_{\pi_x}[c(Y_1, y_0)] = OT_c(P_{1 \mid x}, P_{0 \mid x}), \\
			&E_{\pi_x^H}[c(Y_1, Y_0)] = \theta^H(x) = \sup_{\pi_x \in \Pi(P_{1 \mid x}, P_{0 \mid x})}E_{\pi_x}[c(Y_1, y_0)] = -OT_{-c}(P_{1 \mid x}, P_{0 \mid x})
		\end{align*}
		This shows that there exists a distribution $\pi^L$ of the primitives $(Y_1, Y_0, D, X)$, characterized by $\pi_x^L$ for each $x$ such that $\theta^L = E_{\pi^L}[c(Y_1, Y_0)]$. Similarly, $\theta^H = E_{\pi^H}[c(Y_1, Y_0)]$, and therefore $[\theta^L, \theta^H]$ is the sharp identified set for $\theta$. Moreover, boundedness of $c$ implies $\theta^L(x)$, $\theta^H(x)$, $\theta^L$, and $\theta^H$ are finite.
		
		\item The identified set for $\gamma$, denoted $\Gamma_I$, is $[\gamma^L, \gamma^H]$. 
		
		Since $g(\cdot, \eta)$ is continuous and $[\theta^L, \theta^H]$ is compact, the extreme value theorem implies $\inf_{t \in [\theta^L, \theta^H]} g(t, \eta)$ and $\sup_{t \in [\theta^L, \theta^H]} g(t, \eta)$ are attained and thus $\gamma^L, \gamma^H \in \Gamma_I$. Since $g(\cdot, \eta)$ is continuous, the intermediate value theorem implies every value between $\gamma^L$ and $\gamma^H$ is attained by some value between the corresponding $\argmin$ and $\argmax$. Thus $\Gamma_I = [\gamma^L, \gamma^H]$. 
	\end{enumerate}
\end{proof}


\lemmaSharpnessOfCDFLowerBound*
\begin{proof}
	\singlespacing
	
	The proof is similar to that of lemma \ref{Lemma: identification, function of moments}. In particular, steps one and two of that proof imply the identified set $\Theta_{I, \delta}$ is an interval, and $\theta \in \Theta_{I, \delta}$ if and only if there exists $\pi_x \in \Pi(P_{1 \mid x}, P_{0 \mid x})$ such that $\theta = \sum_{x \in \mathcal{X}} P(X = x)E_{\pi_x}[\mathbbm{1}\{Y_1 - Y_0 \leq \delta\}]$
	
	$\theta^H(\delta)$ is the sharp upper bound. To see this, note that since $c_H(y_1, y_0, \delta) = \mathbbm{1}\{y_1 - y_0 > \delta\}$ is lower semicontinuous and bounded, lemma \ref{Lemma: optimal transport is attained} implies that there exists $\pi_x^H \in \Pi(P_{1 \mid x}, P_{0 \mid x})$ such that $\theta^H(x, \delta) = 1 - P_{\pi_x^H}(Y_1 - Y_0 > \delta) = P_{\pi_x^H}(Y_1 - Y_0 \leq \delta)$. As in the proof of lemma \ref{Lemma: identification, function of moments}, this implies that there exists a distribution $\pi^H$ of the primitives $(Y_1, Y_0, D, X)$ consistent with the identified $P_{d \mid x}$ and $p_{dx} = P(D = d, X = x)$ as well as assumptions \ref{Assumption: setting} and \ref{Assumption: parameter, CDF} such that $\theta^H(\delta) = P_{\pi^H}(Y_1 - Y_0 \leq \delta)$, and thus $\max \Theta_{I, \delta} = \theta^H(\delta)$.
	
	Now consider $\theta^L(\delta)$. $\mathbbm{1}\{y_1 - y_0 < \delta\} \leq \mathbbm{1}\{y_1 - y_0 \leq \delta\}$ implies that 
	\begin{align*}
		\theta^L(x, \delta) = \inf_{\pi_x \in \Pi(P_{1 \mid x}, P_{0 \mid x})} E_{\pi_x}[\mathbbm{1}\{Y_1 - Y_0 < \delta\}] \leq \inf_{\pi_x \in \Pi(P_{1 \mid x}, P_{0 \mid x})} E_{\pi_x}[\mathbbm{1}\{Y_1 - Y_0 \leq \delta\}]
	\end{align*}
	from which it follows that $\theta^L(\delta) = E[\theta^L(X, \delta)]$ is a lower bound on the identified set for $P(Y_1 - Y_0 \leq \delta)$. It suffices to show that there exists $\pi_x^L \in \Pi(P_{1 \mid x}, P_{0 \mid x})$ such that $\theta^L(x, \delta) = P_{\pi_x^L}(Y_1 - Y_0 \leq \delta)$. 
	
	Lemma \ref{Lemma: optimal transport is attained} and corollary \ref{Lemma: duality special case CDF, corollary} implies that there exists $\pi_x^L \in \Pi(P_{1 \mid x}, P_{0 \mid x})$ such that $\theta^L(x) = P_{\pi_x^L}(Y_1 - Y_0 < \delta) = \sup_y \left\{F_{1 \mid x}(y) - F_{0 \mid x}(y - \delta)\right\}$. Moreover, \cite{villani2009optimal} theorem 5.10 part (iii) implies the dual problem $\sup_y \left\{F_{1 \mid x}(y) - F_{0 \mid x}(y - \delta)\right\}$ is attained as well, say by $y^*$. 
	\begin{equation}
		\int \mathbbm{1}\{y_1 - y_0 \leq \delta\} d\pi_x^L(y_1,y_0) = \int \mathbbm{1}\{y_1 \leq y^*\}dP_{1 \mid x}(y_1) - \int \mathbbm{1}\{y_0 \leq y^* - \delta\} dP_{0 \mid x}(y_0) \label{Display: theorem proof, lower bound on CDF is sharp, strong duality}
	\end{equation}
	Next, notice that
	\begin{equation}
		\mathbbm{1}\{y_1 \leq y^*\} - \mathbbm{1}\{y_0 \leq y^* - \delta\} \leq \mathbbm{1}\{y_1 - y_0 < \delta\} \label{Display: theorem proof, lower bound on CDF is sharp, inequality}
	\end{equation}
	which holds for all $(y_1, y_0) \in \mathcal{Y}_1 \times \mathcal{Y}_0$, must hold with equality $\pi_x^L$-almost surely. Indeed, let $N$ be the set where the inequality in \eqref{Display: theorem proof, lower bound on CDF is sharp, inequality} is strict and suppose $N$ is $\pi_x^L$-non-negligible. Since $\pi_x^L \in \Pi(P_{1 \mid x}, P_{0 \mid x})$, 
	\begin{align*}
		&\int \mathbbm{1}\{y_1 \leq y^*\}dP_{1 \mid x}(y_1) - \int \mathbbm{1}\{y_0 \leq y^* - \delta\} dP_{0 \mid x}(y_0) =  \int \mathbbm{1}\{y_1 \leq y^*\} - \mathbbm{1}\{y_0 \leq y^* - \delta\} d\pi_x^L(y_1, y_0) \\
		&= \int_N \mathbbm{1}\{y_1 \leq y^*\} - \mathbbm{1}\{y_0 \leq y^* - \delta\} d\pi_x^L(y_1, y_0) + \int_{N^c} \mathbbm{1}\{y_1 \leq y^*\} - \mathbbm{1}\{y_0 \leq y^* - \delta\} d\pi_x^L(y_1, y_0) \\
		&< \int_N \mathbbm{1}\{y_1 - y_0 < \delta\} d\pi_x^L(y_1, y_0) + \int_{N^c}  \mathbbm{1}\{y_1 - y_0 < \delta\} d\pi_x^L(y_1, y_0) \\
		&= \int \mathbbm{1}\{y_1 - y_0 \leq \delta\} d\pi_x^L(y_1,y_0)
	\end{align*}
	contradicts \eqref{Display: theorem proof, lower bound on CDF is sharp, strong duality}. This implies that have that $\pi_x^L$ concentrates on
	\begin{align*}
		&\left\{(y_1, y_0) \; ; \; y_1 \leq y^*, y_0 > y^* - \delta, y_1 - y_0 < \delta\right\} \cup &&\text{both sides of \eqref{Display: theorem proof, lower bound on CDF is sharp, inequality} equal } 1 \\
		&\left\{(y_1, y_0) \; ; \; y_1 > y^*, y_0 > y^* - \delta, y_1 - y_0 \geq \delta\right\} \cup &&\text{both sides of \eqref{Display: theorem proof, lower bound on CDF is sharp, inequality} equal } 0 \\
		&\left\{(y_1, y_0) \; ; \; y_1 \leq y^*, y_0 \leq y^* - \delta, y_1 - y_0 \geq \delta\right\} &&\text{both sides of \eqref{Display: theorem proof, lower bound on CDF is sharp, inequality} equal } 0
	\end{align*}
	Notice the only point in the set $\{(y_1, y_0) \; ; \; y_1 - y_0 =\delta\}$ where $\pi_x^L$ could put positive mass is the point $(y_1, y_0) = (y^*, y^* - \delta)$. But since $P_{1 \mid x}$ has a continuous CDF,
	\begin{align*}
		0 \leq \pi_x^L(\{(y^*, y^* - \delta)\}) \leq \pi_x^L(\{y^*\} \times \mathcal{Y}_0) = P_{1 \mid x}(\{y^*\}) = 0
	\end{align*}
	Thus $P_{\pi_x^L}(Y_1 - Y_0 = \delta) = 0$, and so $P_{\pi_x^L}(Y_1 - Y_0 \leq \delta) = P_{\pi_x^L}(Y_1 - Y_0 < \delta) = \theta^L(x, \delta)$. 
	
	Apply the preceding argument for each $x \in \mathcal{X}$ to find a distribution $\pi$ of the primitives $(Y_1, Y_0, D, X)$ consistent with assumption \ref{Assumption: setting} and \ref{Assumption: parameter, CDF} such that $\theta^L = P_\pi(Y_1 - Y_0 \leq \delta)$, and thus $\min \Theta_{I,\delta} = \theta^L(\delta)$.
\end{proof}


\lemmaQuantileIdentification*
\begin{proof}
	\singlespacing
	
	Suppose $\theta^L(\gamma) \leq \tau \leq \theta^H(\gamma)$.	Lemma \ref{Lemma: identification, CDF} implies there exists a distribution $\pi$ of the primitives $(Y_1, Y_0, D, X)$ consistent with the identified information and assumptions \ref{Assumption: setting} and \ref{Assumption: parameter, CDF} such that $P_\pi(Y_1 - Y_0 \leq \gamma) = \tau$. Thus $\gamma \in [\sup\{\gamma \; ; \; P_\pi(Y_1 - Y_0 \leq \gamma) < \tau\}, \sup\{\gamma \; ; \; P_\pi(Y_1 - Y_0 \leq \gamma) \leq \tau\}]$ and hence $\gamma \in \Gamma_{I, \tau}$.
	
	Before showing the other direction, we next show that assumption \ref{Assumption: parameter, CDF} implies $\theta^L(\delta)$ is continuous. Specifically, apply corollary \ref{Lemma: duality special case CDF, corollary} to find $\theta^L(\delta, x) = \sup_y \{F_{1 \mid x}(y) - F_{0 \mid x}(y - \delta)\}$. So for any $\delta, \delta'$,  
	\begin{align*}
		\theta^L(\delta, x) - \theta^L(\delta', x) &= \sup_y \{F_{1 \mid x}(y) - F_{0 \mid x}(y - \delta)\} - \sup_y \{F_{1 \mid x}(y) - F_{0 \mid x}(y - \delta')\}  \\
		&\leq \sup_y \left\{F_{0 \mid x}(y - \delta') - F_{0 \mid x}(y - \delta)\right\} \\
		&\leq \sup_y \left\lvert F_{0 \mid x}(y - \delta') - F_{0 \mid x}(y - \delta)\right\rvert
	\end{align*}
	and thus $\lvert \theta^L(\delta, x) - \theta^L(\delta', x) \rvert \leq \sup_y \left\lvert F_{0 \mid x}(y - \delta') - F_{0 \mid x}(y - \delta)\right\rvert$. Recall that any continuous CDF is in fact uniformly continuous, and so $F_{0 \mid x}$ is in fact uniformly continuous. Let $\varepsilon > 0$, choose $\eta > 0$ such that for any $y, y' \in \mathbb{R}$ with $\lvert y - y' \rvert < \eta$, one has $\lvert F_{0 \mid x}(y) - F_{0 \mid x}(y') \rvert < \varepsilon/2$, and notice that 
	\begin{align*}
		\lvert \delta - \delta' \rvert < \eta \implies \sup_y \left\lvert F_{0 \mid x}(y - \delta') - F_{0 \mid x}(y - \delta) \right\rvert \leq \varepsilon/2 < \varepsilon
	\end{align*}
	This shows $\theta^L(\delta,x)$ is continuous, and so $\theta^L(\delta) = E[\theta^L(\delta, X)] = \sum_{x \in \mathcal{X}} P(X = x) \theta^L(x)$ is continuous.
	
	Return to showing the other direction, through the contrapositive. Suppose it is not the case that $\theta^L(\gamma) \leq \tau \leq \theta^H(\gamma)$. There are two possibilities:
	\begin{enumerate}
		\item Suppose $\theta^H(\gamma) < \tau$. Then there is no distribution of the primitives such that $P_\pi(Y_1 - Y_0 \leq \gamma) \geq \tau$, hence there is no distribution where $\gamma \in [\inf\{\gamma \; ; \; P(Y_1 - Y_0 \leq \gamma) \geq \tau\}, \inf\{\gamma \; ; \; P(Y_1 - Y_0 \leq \gamma) > \tau\}]$ and thus $\gamma \not \in \Gamma_{I, \tau}$.
	
		
		\item Suppose $\tau < \theta^L(\gamma)$. If one further supposes that $\gamma \in \Gamma_{I, \tau}$, then $\theta^L(\cdot)$ would have a jump discontinuity at $\gamma$, contradicting the continuity shown above. 
		
		Specifically, if $\tau < \theta^L(\gamma)$, then there exists distributions of the primitives such that $P_\pi(Y_1 - Y_0 \leq \gamma) > \tau$, but none satisfying $P_\pi(Y_1 - Y_0 \leq \gamma) = \tau$. For one of these distributions $\pi$ of the primitives to rationalize $\gamma$ is the $\tau$-th quantile, the CDF of $\pi$ must satisfy
		\begin{equation*}
			\lim_{\epsilon \rightarrow 0} P_\pi(Y_1 - Y_0 \leq \gamma - \epsilon) < \tau < \theta^L(\gamma) \leq P_\pi(Y_1 - Y_0 \leq \gamma)
		\end{equation*}
		i.e., $P_\pi(Y_1 - Y_0 \leq \gamma)$ would have to jump at $\gamma$ from below $\tau$ to above $\theta^L(\gamma)$, a jump discontinuity at $\gamma$ of at least $\varepsilon = \theta^L(\gamma) - \tau > 0$. But then $\theta^L(\cdot)$ would have a jump discontinuity of at least $\varepsilon$ at $\gamma$. 
	\end{enumerate}
	In either case, $\gamma \not \in \Gamma_{I, \tau}$. This completes the proof.
\end{proof}
